# Supplementary material for: Jiamusi pulsar observations: III. Nulling of 20 pulsars
Source: arXiv:2009.08637 source file (2020-09-18)
Supplement: Supplementary file 1 [file appendix.b.tex]

\appendix

%%%%%%%%%%%%%%%%%%%%%%%%%%%%%%%%%
\section{Nulling pulsars reported previously}

\input table_p.tex

%\clearpage

\section{Nulling behaviours of 20 pulsars}

\twocolumn

%%%%%%%%%%%%
\clearpage
\newsavebox{\bigimage}
%%%%%%%%%%%%%%%%%%%%%%%%%%%%%%%%%
%%%%%%%%%%%%%%%%%%%%%%% J0034
\begin{figure}
  \centering
  \sbox{\bigimage}{%
    \begin{subfigure}[b]{.2\textwidth}
      \centering
      \includegraphics[height=1.21cm, width=0.8\textwidth]{J0034-0721_2015-12-12_S8_A_NF_dis.ps}
      \caption{\scriptsize Nulling fraction}
      %\vfill
      \includegraphics[height=7.0cm, width=0.8\textwidth]{J0034-0721_2015-12-12_S8_A_Phase_t.ps}
      \caption{\scriptsize Pulse sequence and states}
      \includegraphics[height=1.0cm,width=0.7\textwidth]{J0034-0721_2015-12-12_S8_A_B_profs.ps}
      \caption{\scriptsize Integrated pulse profiles}
      \vspace{0pt}% reference point at the very bottom
    \end{subfigure}%
  }
  \usebox{\bigimage}
  %\hfill
  \begin{minipage}[b][\ht\bigimage][s]{.2\textwidth}
    \begin{subfigure}{\textwidth}
      \centering
      \includegraphics[height=1.8cm, width=0.8\textwidth]{J0034-0721_2015-12-12_S8_A_BN_dis.ps}
      \caption{\scriptsize Burst and Null lengths}
    \end{subfigure}%
    \vfill
    \begin{subfigure}{\textwidth}
      \centering
      \includegraphics[height=1.8cm, width=0.8\textwidth]{J0034-0721_2015-12-12_S8_A_BN_cor.ps}
      \caption{\scriptsize Brust and Null interaction}
    \end{subfigure}
    \vfill
    \begin{subfigure}{\textwidth}
      \centering
      \includegraphics[height=3.0cm,width=0.7\textwidth]{J0034-0721_2015-12-12_S8_A_BN_period.ps}
      \caption{\scriptsize Nulling periodicity}
    \end{subfigure}
    \vfill
    \begin{subfigure}{\textwidth}
      \centering
      \includegraphics[height=1.7cm,width=0.8\textwidth]{J0034-0721_2015-12-12_S8_A_BE_decay.ps}
      \caption{\scriptsize Variation of burst intensities}
    \end{subfigure}
    \vspace{0pt}% reference point at the very bottom
  \end{minipage}
  \caption{PSR J0034-0721 observed on 2015-12-12 A.}
  \label{fig:J0034A}
\end{figure}

\begin{figure}
  \centering
  \sbox{\bigimage}{%
    \begin{subfigure}[b]{.2\textwidth}
      \centering
      \includegraphics[height=1.21cm, width=0.8\textwidth]{J0034-0721_2015-12-12_S8_B_NF_dis.ps}
      \caption{\scriptsize Nulling fraction}
      %\vfill
      \includegraphics[height=7.0cm, width=0.8\textwidth]{J0034-0721_2015-12-12_S8_B_Phase_t.ps}
      \caption{\scriptsize Pulse sequence and states}
      \includegraphics[height=1.0cm,width=0.7\textwidth]{J0034-0721_2015-12-12_S8_B_B_profs.ps}
      \caption{\scriptsize Integrated pulse profiles}
      \vspace{0pt}% reference point at the very bottom
    \end{subfigure}%
  }
  \usebox{\bigimage}
  %\hfill
  \begin{minipage}[b][\ht\bigimage][s]{.2\textwidth}
    \begin{subfigure}{\textwidth}
      \centering
      \includegraphics[height=1.8cm, width=0.8\textwidth]{J0034-0721_2015-12-12_S8_B_BN_dis.ps}
      \caption{\scriptsize Burst and Null lengths}
    \end{subfigure}%
    \vfill
    \begin{subfigure}{\textwidth}
      \centering
      \includegraphics[height=1.8cm, width=0.8\textwidth]{J0034-0721_2015-12-12_S8_B_BN_cor.ps}
      \caption{\scriptsize Brust and Null interaction}
    \end{subfigure}
    \vfill
    \begin{subfigure}{\textwidth}
      \centering
      \includegraphics[height=3.0cm,width=0.7\textwidth]{J0034-0721_2015-12-12_S8_B_BN_period.ps}
      \caption{\scriptsize Nulling periodicity}
    \end{subfigure}
    \vfill
    \begin{subfigure}{\textwidth}
      \centering
      \includegraphics[height=1.7cm,width=0.8\textwidth]{J0034-0721_2015-12-12_S8_B_BE_decay.ps}
      \caption{\scriptsize Variation of burst intensities}
    \end{subfigure}
    \vspace{0pt}% reference point at the very bottom
  \end{minipage}
  \caption{PSR J0034-0721 observed on 2015-12-12 B.}
  \label{fig:J0034B}
\end{figure}

%%%%%%%%%%%%%%%%%%%%%%%%%%%%%%%%%%%%%%%%%%%%%%%%%%%%%%%%%%%%%%%%%%%%%%%%%%%%%%%%%%%%%%%%%% J0248
\begin{figure}
  \centering
  \sbox{\bigimage}{%
    \begin{subfigure}[b]{.2\textwidth}
      \centering
      \includegraphics[height=1.21cm, width=0.8\textwidth]{J0248+6021_2015-06-16_S8_0_NF_dis.ps}
      \caption{\scriptsize Nulling fraction}
      %\vfill
      \includegraphics[height=7.0cm, width=0.8\textwidth]{J0248+6021_2015-06-16_S8_0_Phase_t.ps}
      \caption{\scriptsize Pulse sequence and states}
      \includegraphics[height=1.0cm,width=0.7\textwidth]{J0248+6021_2015-06-16_S8_0_B_profs.ps}
      \caption{\scriptsize Integrated pulse profiles}
      \vspace{0pt}% reference point at the very bottom
    \end{subfigure}%
  }
  \usebox{\bigimage}
  %\hfill
  \begin{minipage}[b][\ht\bigimage][s]{.2\textwidth}
    \begin{subfigure}{\textwidth}
      \centering
      \includegraphics[height=1.8cm, width=0.8\textwidth]{J0248+6021_2015-06-16_S8_0_BN_dis.ps}
      \caption{\scriptsize Burst and Null lengths}
    \end{subfigure}%
    \vfill
    \begin{subfigure}{\textwidth}
      \centering
      \includegraphics[height=1.8cm, width=0.8\textwidth]{J0248+6021_2015-06-16_S8_0_BN_cor.ps}
      \caption{\scriptsize Brust and Null interaction}
    \end{subfigure}
    \vfill
    \begin{subfigure}{\textwidth}
      \centering
      \includegraphics[height=3.0cm,width=0.7\textwidth]{J0248+6021_2015-06-16_S8_0_BN_period.ps}
      \caption{\scriptsize Nulling periodicity}
    \end{subfigure}
    \vfill
    \begin{subfigure}{\textwidth}
      \centering
      \includegraphics[height=1.7cm,width=0.8\textwidth]{J0248+6021_2015-06-16_S8_0_BE_decay.ps}
      \caption{\scriptsize Variation of burst intensities}
    \end{subfigure}
    \vspace{0pt}% reference point at the very bottom
  \end{minipage}
  \caption{PSR J0248+6021 observed on 2015-06-16.}
  \label{fig:J0248_20150616}
\end{figure}

\begin{figure}
  \centering
  \sbox{\bigimage}{%
    \begin{subfigure}[b]{.2\textwidth}
      \centering
      \includegraphics[height=1.21cm, width=0.8\textwidth]{J0248+6021_2016-08-11_S8_0_NF_dis.ps}
      \caption{\scriptsize Nulling fraction}
      %\vfill
      \includegraphics[height=7.0cm, width=0.8\textwidth]{J0248+6021_2016-08-11_S8_0_Phase_t.ps}
      \caption{\scriptsize Pulse sequence and states}
      \includegraphics[height=1.0cm,width=0.7\textwidth]{J0248+6021_2016-08-11_S8_0_B_profs.ps}
      \caption{\scriptsize Integrated pulse profiles}
      \vspace{0pt}% reference point at the very bottom
    \end{subfigure}%
  }
  \usebox{\bigimage}
  %\hfill
  \begin{minipage}[b][\ht\bigimage][s]{.2\textwidth}
    \begin{subfigure}{\textwidth}
      \centering
      \includegraphics[height=1.8cm, width=0.8\textwidth]{J0248+6021_2016-08-11_S8_0_BN_dis.ps}
      \caption{\scriptsize Burst and Null lengths}
    \end{subfigure}%
    \vfill
    \begin{subfigure}{\textwidth}
      \centering
      \includegraphics[height=1.8cm, width=0.8\textwidth]{J0248+6021_2016-08-11_S8_0_BN_cor.ps}
      \caption{\scriptsize Brust and Null interaction}
    \end{subfigure}
    \vfill
    \begin{subfigure}{\textwidth}
      \centering
      \includegraphics[height=3.0cm,width=0.7\textwidth]{J0248+6021_2016-08-11_S8_0_BN_period.ps}
      \caption{\scriptsize Nulling periodicity}
    \end{subfigure}
    \vfill
    \begin{subfigure}{\textwidth}
      \centering
      \includegraphics[height=1.7cm,width=0.8\textwidth]{J0248+6021_2016-08-11_S8_0_BE_decay.ps}
      \caption{\scriptsize Variation of burst intensities}
    \end{subfigure}
    \vspace{0pt}% reference point at the very bottom
  \end{minipage}
  \caption{PSR J0248+6021 observed on 2016-08-11.}
  \label{fig:J0248_20160811}
\end{figure}

%%%%%%%%%%%%%%%%%%%%%%%%%%%%%%%%%%%%%%%%%%%%%%%%%%%%%%%%%%%%%%%%%%%%%%%%%%%%%%%%%%%%%%%%%%%%%%%%%% J0304
\begin{figure}
  \centering
  \sbox{\bigimage}{%
    \begin{subfigure}[b]{.2\textwidth}
      \centering
      \includegraphics[height=1.21cm, width=0.8\textwidth]{J0304+1932_2015-12-14_S8_0_NF_dis.ps}
      \caption{\scriptsize Nulling fraction}
      %\vfill
      \includegraphics[height=7.0cm, width=0.8\textwidth]{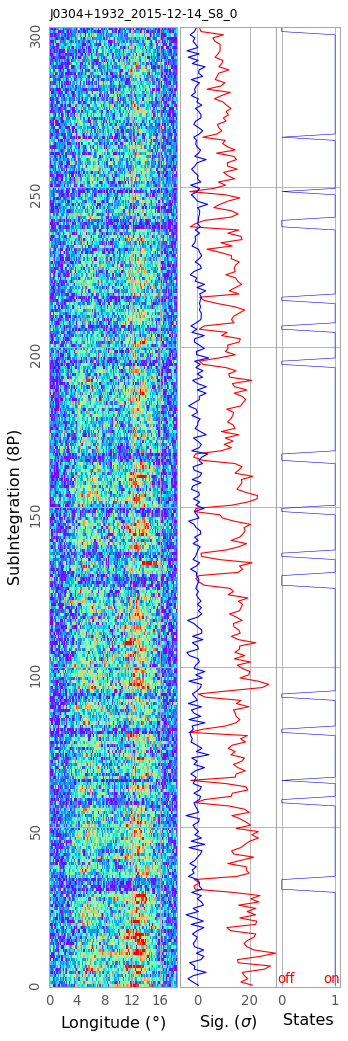}
      \caption{\scriptsize Pulse sequence and states}
      \includegraphics[height=1.0cm,width=0.7\textwidth]{J0304+1932_2015-12-14_S8_0_B_profs.ps}
      \caption{\scriptsize Integrated pulse profiles}
      \vspace{0pt}% reference point at the very bottom
    \end{subfigure}%
  }
  \usebox{\bigimage}
  %\hfill
  \begin{minipage}[b][\ht\bigimage][s]{.2\textwidth}
    \begin{subfigure}{\textwidth}
      \centering
      \includegraphics[height=1.8cm, width=0.8\textwidth]{J0304+1932_2015-12-14_S8_0_BN_dis.ps}
      \caption{\scriptsize Burst and Null lengths}
    \end{subfigure}%
    \vfill
    \begin{subfigure}{\textwidth}
      \centering
      \includegraphics[height=1.8cm, width=0.8\textwidth]{J0304+1932_2015-12-14_S8_0_BN_cor.ps}
      \caption{\scriptsize Brust and Null interaction}
    \end{subfigure}
    \vfill
    \begin{subfigure}{\textwidth}
      \centering
      \includegraphics[height=3.0cm,width=0.7\textwidth]{J0304+1932_2015-12-14_S8_0_BN_period.ps}
      \caption{\scriptsize Nulling periodicity}
    \end{subfigure}
    \vfill
    \begin{subfigure}{\textwidth}
      \centering
      \includegraphics[height=1.7cm,width=0.8\textwidth]{J0304+1932_2015-12-14_S8_0_BE_decay.ps}
      \caption{\scriptsize Variation of burst intensities}
    \end{subfigure}
    \vspace{0pt}% reference point at the very bottom
  \end{minipage}
  \caption{PSR J0304+1932 observed on 2015-12-14.}
  \label{fig:J0304_20151214}
\end{figure}
%%%%%%%%%%%%%%%%%%%%%%%%%%%%%%%%%%%%%%%%%%%%%%%%%%%%%%%%%%%%%%%%%%%%%%%%%%%%%%%%%%%%%%%%%%%%%% J0332
\begin{figure}
  \centering
  \sbox{\bigimage}{%
    \begin{subfigure}[b]{.2\textwidth}
      \centering
      \includegraphics[height=1.21cm, width=0.8\textwidth]{J0332+5434_2016-02-21_S1_A_NF_dis.ps}
      \caption{\scriptsize Nulling fraction}
      %\vfill
      \includegraphics[height=7.0cm, width=0.8\textwidth]{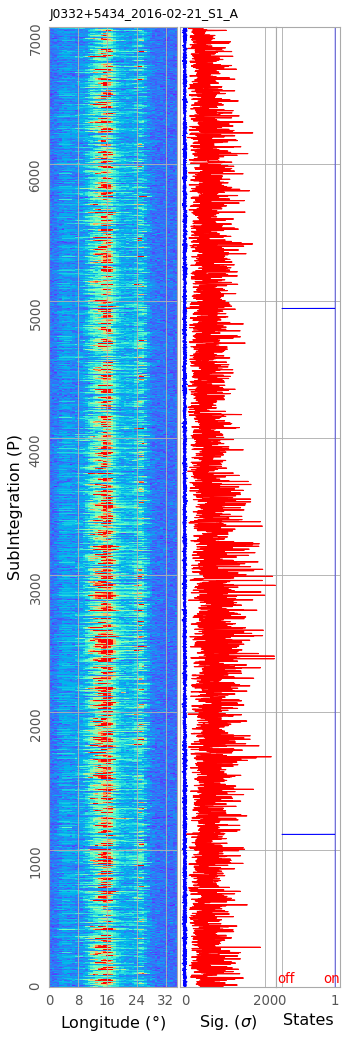}
      \caption{\scriptsize Pulse sequence and states}
      \vspace{0pt}% reference point at the very bottom
    \end{subfigure}%
  }
  \usebox{\bigimage}
  %\hfill
  \begin{minipage}[b][\ht\bigimage][s]{.2\textwidth}
    \vfill 
    \vspace{0pt}% reference point at the very bottom
  \end{minipage}
  \caption{PSR J0332+5434 observed on 2016-02-21A.}
  \label{fig:J0332_20160221A}
\end{figure}

\begin{figure}
  \centering
  \sbox{\bigimage}{%
    \begin{subfigure}[b]{.2\textwidth}
      \centering
      \includegraphics[height=1.21cm, width=0.8\textwidth]{J0332+5434_2016-02-21_S1_B_NF_dis.ps}
      \caption{\scriptsize Nulling fraction}
      %\vfill
      \includegraphics[height=7.0cm, width=0.8\textwidth]{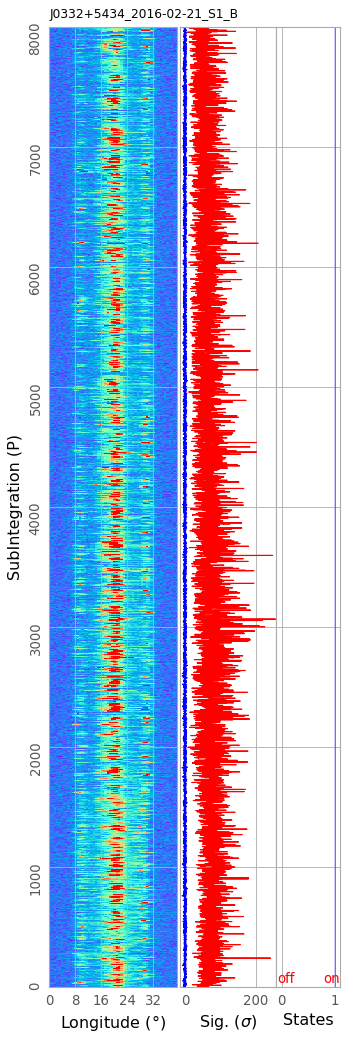}
      \caption{\scriptsize Pulse sequence and states}
      \vspace{0pt}% reference point at the very bottom
    \end{subfigure}%
  }
    \usebox{\bigimage}
  %\hfill
  \begin{minipage}[b][\ht\bigimage][s]{.2\textwidth}
    \vfill 
    \vspace{0pt}% reference point at the very bottom
  \end{minipage}
  \caption{PSR J0332+5434 observed on 2016-02-21B.}
  \label{fig:J0332_20160221B}
\end{figure}

\begin{figure}
  \centering
  \sbox{\bigimage}{%
    \begin{subfigure}[b]{.2\textwidth}
      \centering
      \includegraphics[height=1.21cm, width=0.8\textwidth]{J0332+5434_2016-02-24_S1_0_NF_dis.ps}
      \caption{\scriptsize Nulling fraction}
      %\vfill
      \includegraphics[height=7.0cm, width=0.8\textwidth]{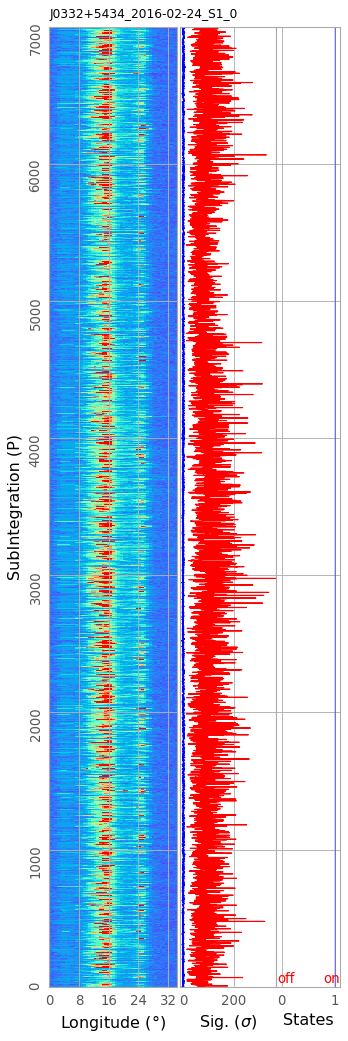}
      \caption{\scriptsize Pulse sequence and states}
      \vspace{0pt}% reference point at the very bottom
    \end{subfigure}%
  }
    \usebox{\bigimage}
  %\hfill
  \begin{minipage}[b][\ht\bigimage][s]{.2\textwidth}
    \vfill 
    \vspace{0pt}% reference point at the very bottom
  \end{minipage}
  \caption{PSR J0332+5434 observed on 2016-02-24.}
  \label{fig:J0332_20160224}
\end{figure}

%%%%%%%%%%%%%%%%%%%%%%%%%%%%%%%%%%%%%%%%%%%%%%%%%%%%%%%%%%%%%%%%%%%%%%%%%%%%%%%%%%%%%%%%%%%%%% J0528
\begin{figure}
  \centering
  \sbox{\bigimage}{%
    \begin{subfigure}[b]{.2\textwidth}
      \centering
      \includegraphics[height=1.21cm, width=0.8\textwidth]{J0528+2200_2015-06-18_S1_0_NF_dis.ps}
      \caption{\scriptsize Nulling fraction}
      %\vfill
      \includegraphics[height=7.0cm, width=0.8\textwidth]{J0528+2200_2015-06-18_S1_0_Phase_t.ps}
      \caption{\scriptsize Pulse sequence and states}
      \includegraphics[height=1.0cm,width=0.7\textwidth]{J0528+2200_2015-06-18_S1_0_B_profs.ps}
      \caption{\scriptsize Integrated pulse profiles}
      \vspace{0pt}% reference point at the very bottom
    \end{subfigure}%
  }
  \usebox{\bigimage}
  %\hfill
  \begin{minipage}[b][\ht\bigimage][s]{.2\textwidth}
    \begin{subfigure}{\textwidth}
      \centering
      \includegraphics[height=1.8cm, width=0.8\textwidth]{J0528+2200_2015-06-18_S1_0_BN_dis.ps}
      \caption{\scriptsize Burst and Null lengths}
    \end{subfigure}%
    \vfill
    \begin{subfigure}{\textwidth}
      \centering
      \includegraphics[height=1.8cm, width=0.8\textwidth]{J0528+2200_2015-06-18_S1_0_BN_cor.ps}
      \caption{\scriptsize Brust and Null interaction}
    \end{subfigure}
    \vfill
    \begin{subfigure}{\textwidth}
      \centering
      \includegraphics[height=3.0cm,width=0.7\textwidth]{J0528+2200_2015-06-18_S1_0_BN_period.ps}
      \caption{\scriptsize Nulling periodicity}
    \end{subfigure}
    \vfill
    \begin{subfigure}{\textwidth}
      \centering
      \includegraphics[height=1.7cm,width=0.8\textwidth]{J0528+2200_2015-06-18_S1_0_BE_decay.ps}
      \caption{\scriptsize Variation of burst intensities}
    \end{subfigure}
    \vspace{0pt}% reference point at the very bottom
  \end{minipage}
  \caption{PSR J0528+2200 observed on 2015-06-18.}
  \label{fig:J0528_20150618}
\end{figure}

\begin{figure}
  \centering
  \sbox{\bigimage}{%
    \begin{subfigure}[b]{.2\textwidth}
      \centering
      \includegraphics[height=1.21cm, width=0.8\textwidth]{J0528+2200_2016-01-27_S1_0_NF_dis.ps}
      \caption{\scriptsize Nulling fraction}
      %\vfill
      \includegraphics[height=7.0cm, width=0.8\textwidth]{J0528+2200_2016-01-27_S1_0_Phase_t.ps}
      \caption{\scriptsize Pulse sequence and states}
      \includegraphics[height=1.0cm,width=0.7\textwidth]{J0528+2200_2016-01-27_S1_0_B_profs.ps}
      \caption{\scriptsize Integrated pulse profiles}
      \vspace{0pt}% reference point at the very bottom
    \end{subfigure}%
  }
  \usebox{\bigimage}
  %\hfill
  \begin{minipage}[b][\ht\bigimage][s]{.2\textwidth}
    \begin{subfigure}{\textwidth}
      \centering
      \includegraphics[height=1.8cm, width=0.8\textwidth]{J0528+2200_2016-01-27_S1_0_BN_dis.ps}
      \caption{\scriptsize Burst and Null lengths}
    \end{subfigure}%
    \vfill
    \begin{subfigure}{\textwidth}
      \centering
      \includegraphics[height=1.8cm, width=0.8\textwidth]{J0528+2200_2016-01-27_S1_0_BN_cor.ps}
      \caption{\scriptsize Brust and Null interaction}
    \end{subfigure}
    \vfill
    \begin{subfigure}{\textwidth}
      \centering
      \includegraphics[height=3.0cm,width=0.7\textwidth]{J0528+2200_2016-01-27_S1_0_BN_period.ps}
      \caption{\scriptsize Nulling periodicity}
    \end{subfigure}
    \vfill
    \begin{subfigure}{\textwidth}
      \centering
      \includegraphics[height=1.7cm,width=0.8\textwidth]{J0528+2200_2016-01-27_S1_0_BE_decay.ps}
      \caption{\scriptsize Variation of burst intensities}
    \end{subfigure}
    \vspace{0pt}% reference point at the very bottom
  \end{minipage}
  \caption{PSR J0528+2200 observed on 2016-01-27.}
  \label{fig:J0528_20160127}
\end{figure}

%%%%%%%%%%%%%%%%%%%%%%%%%%%%%%%%%%%%%%%%%%%%%%%%%%%%%%%%%%%%%%%%%%%%%%%%%%%%%%%%%%%%%%%%%%%%%% J0543
\begin{figure}
  \centering
  \sbox{\bigimage}{%
    \begin{subfigure}[b]{.2\textwidth}
      \centering
      \includegraphics[height=1.21cm, width=0.8\textwidth]{J0543+2329_2015-06-25_S4_0_NF_dis.ps}
      \caption{\scriptsize Nulling fraction}
      %\vfill
      \includegraphics[height=7.0cm, width=0.8\textwidth]{J0543+2329_2015-06-25_S4_0_Phase_t.ps}
      \caption{\scriptsize Pulse sequence and states}
      \includegraphics[height=1.0cm,width=0.7\textwidth]{J0543+2329_2015-06-25_S4_0_B_profs.ps}
      \caption{\scriptsize Integrated pulse profiles}
      \vspace{0pt}% reference point at the very bottom
    \end{subfigure}%
  }
  \usebox{\bigimage}
  %\hfill
  \begin{minipage}[b][\ht\bigimage][s]{.2\textwidth}
    \begin{subfigure}{\textwidth}
      \centering
      \includegraphics[height=1.8cm, width=0.8\textwidth]{J0543+2329_2015-06-25_S4_0_BN_dis.ps}
      \caption{\scriptsize Burst and Null lengths}
    \end{subfigure}%
    \vfill
    \begin{subfigure}{\textwidth}
      \centering
      \includegraphics[height=1.8cm, width=0.8\textwidth]{J0543+2329_2015-06-25_S4_0_BN_cor.ps}
      \caption{\scriptsize Brust and Null interaction}
    \end{subfigure}
    \vfill
    \begin{subfigure}{\textwidth}
      \centering
      \includegraphics[height=3.0cm,width=0.7\textwidth]{J0543+2329_2015-06-25_S4_0_BN_period.ps}
      \caption{\scriptsize Nulling periodicity}
    \end{subfigure}
    \vfill
    \begin{subfigure}{\textwidth}
      \centering
      \includegraphics[height=1.7cm,width=0.8\textwidth]{J0543+2329_2015-06-25_S4_0_BE_decay.ps}
      \caption{\scriptsize Variation of burst intensities}
    \end{subfigure}
    \vspace{0pt}% reference point at the very bottom
  \end{minipage}
  \caption{PSR J0543+2329 observed on 2015-06-25.}
  \label{fig:J0543_20150625}
\end{figure}

\begin{figure}
  \centering
  \sbox{\bigimage}{%
    \begin{subfigure}[b]{.2\textwidth}
      \centering
      \includegraphics[height=1.21cm, width=0.8\textwidth]{J0543+2329_2017-11-01_S4_A_NF_dis.ps}
      \caption{\scriptsize Nulling fraction}
      %\vfill
      \includegraphics[height=7.0cm, width=0.8\textwidth]{J0543+2329_2017-11-01_S4_A_Phase_t.ps}
      \caption{\scriptsize Pulse sequence and states}
      \includegraphics[height=1.0cm,width=0.7\textwidth]{J0543+2329_2017-11-01_S4_A_B_profs.ps}
      \caption{\scriptsize Integrated pulse profiles}
      \vspace{0pt}% reference point at the very bottom
    \end{subfigure}%
  }
  \usebox{\bigimage}
  %\hfill
  \begin{minipage}[b][\ht\bigimage][s]{.2\textwidth}
    \begin{subfigure}{\textwidth}
      \centering
      \includegraphics[height=1.8cm, width=0.8\textwidth]{J0543+2329_2017-11-01_S4_A_BN_dis.ps}
      \caption{\scriptsize Burst and Null lengths}
    \end{subfigure}%
    \vfill
    \begin{subfigure}{\textwidth}
      \centering
      \includegraphics[height=1.8cm, width=0.8\textwidth]{J0543+2329_2017-11-01_S4_A_BN_cor.ps}
      \caption{\scriptsize Brust and Null interaction}
    \end{subfigure}
    \vfill
    \begin{subfigure}{\textwidth}
      \centering
      \includegraphics[height=3.0cm,width=0.7\textwidth]{J0543+2329_2017-11-01_S4_A_BN_period.ps}
      \caption{\scriptsize Nulling periodicity}
    \end{subfigure}
    \vfill
    \begin{subfigure}{\textwidth}
      \centering
      \includegraphics[height=1.7cm,width=0.8\textwidth]{J0543+2329_2017-11-01_S4_A_BE_decay.ps}
      \caption{\scriptsize Variation of burst intensities}
    \end{subfigure}
    \vspace{0pt}% reference point at the very bottom
  \end{minipage}
  \caption{PSR J0543+2329 observed on 2017-11-01 A.}
  \label{fig:J0543_20171101A}
\end{figure}

\begin{figure}
  \centering
  \sbox{\bigimage}{%
    \begin{subfigure}[b]{.2\textwidth}
      \centering
      \includegraphics[height=1.21cm, width=0.8\textwidth]{J0543+2329_2017-11-01_S4_B_NF_dis.ps}
      \caption{\scriptsize Nulling fraction}
      %\vfill
      \includegraphics[height=7.0cm, width=0.8\textwidth]{J0543+2329_2017-11-01_S4_B_Phase_t.ps}
      \caption{\scriptsize Pulse sequence and states}
      \includegraphics[height=1.0cm,width=0.7\textwidth]{J0543+2329_2017-11-01_S4_B_B_profs.ps}
      \caption{\scriptsize Integrated pulse profiles}
      \vspace{0pt}% reference point at the very bottom
    \end{subfigure}%
  }
  \usebox{\bigimage}
  %\hfill
  \begin{minipage}[b][\ht\bigimage][s]{.2\textwidth}
    \begin{subfigure}{\textwidth}
      \centering
      \includegraphics[height=1.8cm, width=0.8\textwidth]{J0543+2329_2017-11-01_S4_B_BN_dis.ps}
      \caption{\scriptsize Burst and Null lengths}
    \end{subfigure}%
    \vfill
    \begin{subfigure}{\textwidth}
      \centering
      \includegraphics[height=1.8cm, width=0.8\textwidth]{J0543+2329_2017-11-01_S4_B_BN_cor.ps}
      \caption{\scriptsize Brust and Null interaction}
    \end{subfigure}
    \vfill
    \begin{subfigure}{\textwidth}
      \centering
      \includegraphics[height=3.0cm,width=0.7\textwidth]{J0543+2329_2017-11-01_S4_B_BN_period.ps}
      \caption{\scriptsize Nulling periodicity}
    \end{subfigure}
    \vfill
    \begin{subfigure}{\textwidth}
      \centering
      \includegraphics[height=1.7cm,width=0.8\textwidth]{J0543+2329_2017-11-01_S4_B_BE_decay.ps}
      \caption{\scriptsize Variation of burst intensities}
    \end{subfigure}
    \vspace{0pt}% reference point at the very bottom
  \end{minipage}
  \caption{PSR J0543+2329 observed on 2017-11-01 B.}
  \label{fig:J0543_20171101B}
\end{figure}

%%%%%%%%%%%%%%%%%%%%%%%%%%%%%%%%%%%%%%%%%%%%%%%%%%%%%%%%%%%%%%%%%%%%%%%%%%%%%%%%%%%%%%%%%%%%%%%%% J0826
\begin{figure}
  \centering
  \sbox{\bigimage}{%
    \begin{subfigure}[b]{.2\textwidth}
      \centering
      \includegraphics[height=1.21cm, width=0.8\textwidth]{J0826+2637_2015-11-12_S1_A_NF_dis.ps}
      \caption{\scriptsize Nulling fraction}
      %\vfill
      \includegraphics[height=7.0cm, width=0.8\textwidth]{J0826+2637_2015-11-12_S1_A_Phase_t.ps}
      \caption{\scriptsize Pulse sequence and states}
      \includegraphics[height=1.0cm,width=0.7\textwidth]{J0826+2637_2015-11-12_S1_A_B_profs.ps}
      \caption{\scriptsize Integrated pulse profiles}
      \vspace{0pt}% reference point at the very bottom
    \end{subfigure}%
  }
  \usebox{\bigimage}
  %\hfill
  \begin{minipage}[b][\ht\bigimage][s]{.2\textwidth}
    \begin{subfigure}{\textwidth}
      \centering
      \includegraphics[height=1.8cm, width=0.8\textwidth]{J0826+2637_2015-11-12_S1_A_BN_dis.ps}
      \caption{\scriptsize Burst and Null lengths}
    \end{subfigure}%
    \vfill
    \begin{subfigure}{\textwidth}
      \centering
      \includegraphics[height=1.8cm, width=0.8\textwidth]{J0826+2637_2015-11-12_S1_A_BN_cor.ps}
      \caption{\scriptsize Brust and Null interaction}
    \end{subfigure}
    \vfill
    \begin{subfigure}{\textwidth}
      \centering
      \includegraphics[height=3.0cm,width=0.7\textwidth]{J0826+2637_2015-11-12_S1_A_BN_period.ps}
      \caption{\scriptsize Nulling periodicity}
    \end{subfigure}
    \vfill
    \begin{subfigure}{\textwidth}
      \centering
      \includegraphics[height=1.7cm,width=0.8\textwidth]{J0826+2637_2015-11-12_S1_A_BE_decay.ps}
      \caption{\scriptsize Variation of burst intensities}
    \end{subfigure}
    \vspace{0pt}% reference point at the very bottom
  \end{minipage}
  \caption{PSR J0826+2637 observed on 2015-11-12 A.}
  \label{fig:J0826_20151112A}
\end{figure}

\begin{figure}
  \centering
  \sbox{\bigimage}{%
    \begin{subfigure}[b]{.2\textwidth}
      \centering
      \includegraphics[height=1.21cm, width=0.8\textwidth]{J0826+2637_2015-11-12_S1_B_NF_dis.ps}
      \caption{\scriptsize Nulling fraction}
      %\vfill
      \includegraphics[height=7.0cm, width=0.8\textwidth]{J0826+2637_2015-11-12_S1_B_Phase_t.ps}
      \caption{\scriptsize Pulse sequence and states}
      \includegraphics[height=1.0cm,width=0.7\textwidth]{J0826+2637_2015-11-12_S1_B_B_profs.ps}
      \caption{\scriptsize Integrated pulse profiles}
      \vspace{0pt}% reference point at the very bottom
    \end{subfigure}%
  }
  \usebox{\bigimage}
  %\hfill
  \begin{minipage}[b][\ht\bigimage][s]{.2\textwidth}
    \begin{subfigure}{\textwidth}
      \centering
      \includegraphics[height=1.8cm, width=0.8\textwidth]{J0826+2637_2015-11-12_S1_B_BN_dis.ps}
      \caption{\scriptsize Burst and Null lengths}
    \end{subfigure}%
    \vfill
    \begin{subfigure}{\textwidth}
      \centering
      \includegraphics[height=1.8cm, width=0.8\textwidth]{J0826+2637_2015-11-12_S1_B_BN_cor.ps}
      \caption{\scriptsize Brust and Null interaction}
    \end{subfigure}
    \vfill
    \begin{subfigure}{\textwidth}
      \centering
      \includegraphics[height=3.0cm,width=0.7\textwidth]{J0826+2637_2015-11-12_S1_B_BN_period.ps}
      \caption{\scriptsize Nulling periodicity}
    \end{subfigure}
    \vfill
    \begin{subfigure}{\textwidth}
      \centering
      \includegraphics[height=1.7cm,width=0.8\textwidth]{J0826+2637_2015-11-12_S1_B_BE_decay.ps}
      \caption{\scriptsize Variation of burst intensities}
    \end{subfigure}
    \vspace{0pt}% reference point at the very bottom
  \end{minipage}
  \caption{PSR J0826+2637 observed on 2015-11-12 B.}
  \label{fig:J0826_20151112B}
\end{figure}

\begin{figure}
  \centering
  \sbox{\bigimage}{%
    \begin{subfigure}[b]{.2\textwidth}
      \centering
      \includegraphics[height=1.21cm, width=0.8\textwidth]{J0826+2637_2015-11-14_S1_A_NF_dis.ps}
      \caption{\scriptsize Nulling fraction}
      %\vfill
      \includegraphics[height=7.0cm, width=0.8\textwidth]{J0826+2637_2015-11-14_S1_A_Phase_t.ps}
      \caption{\scriptsize Pulse sequence and states}
      \includegraphics[height=1.0cm,width=0.7\textwidth]{J0826+2637_2015-11-14_S1_A_B_profs.ps}
      \caption{\scriptsize Integrated pulse profiles}
      \vspace{0pt}% reference point at the very bottom
    \end{subfigure}%
  }
  \usebox{\bigimage}
  %\hfill
  \begin{minipage}[b][\ht\bigimage][s]{.2\textwidth}
    \begin{subfigure}{\textwidth}
      \centering
      \includegraphics[height=1.8cm, width=0.8\textwidth]{J0826+2637_2015-11-14_S1_A_BN_dis.ps}
      \caption{\scriptsize Burst and Null lengths}
    \end{subfigure}%
    \vfill
    \begin{subfigure}{\textwidth}
      \centering
      \includegraphics[height=1.8cm, width=0.8\textwidth]{J0826+2637_2015-11-14_S1_A_BN_cor.ps}
      \caption{\scriptsize Brust and Null interaction}
    \end{subfigure}
    \vfill
    \begin{subfigure}{\textwidth}
      \centering
      \includegraphics[height=3.0cm,width=0.7\textwidth]{J0826+2637_2015-11-14_S1_A_BN_period.ps}
      \caption{\scriptsize Nulling periodicity}
    \end{subfigure}
    \vfill
    \begin{subfigure}{\textwidth}
      \centering
      \includegraphics[height=1.7cm,width=0.8\textwidth]{J0826+2637_2015-11-14_S1_A_BE_decay.ps}
      \caption{\scriptsize Variation of burst intensities}
    \end{subfigure}
    \vspace{0pt}% reference point at the very bottom
  \end{minipage}
  \caption{PSR J0826+2637 observed on 2015-11-14 A.}
  \label{fig:J0826_20151114A}
\end{figure}
%%%%%%%%%%%%
\clearpage
%%%%%%%%%%%%
\begin{figure}
  \centering
  \sbox{\bigimage}{%
    \begin{subfigure}[b]{.2\textwidth}
      \centering
      \includegraphics[height=1.21cm, width=0.8\textwidth]{J0826+2637_2015-11-14_S1_B_NF_dis.ps}
      \caption{\scriptsize Nulling fraction}
      %\vfill
      \includegraphics[height=7.0cm, width=0.8\textwidth]{J0826+2637_2015-11-14_S1_B_Phase_t.ps}
      \caption{\scriptsize Pulse sequence and states}
      \includegraphics[height=1.0cm,width=0.7\textwidth]{J0826+2637_2015-11-14_S1_B_B_profs.ps}
      \caption{\scriptsize Integrated pulse profiles}
      \vspace{0pt}% reference point at the very bottom
    \end{subfigure}%
  }
  \usebox{\bigimage}
  %\hfill
  \begin{minipage}[b][\ht\bigimage][s]{.2\textwidth}
    \begin{subfigure}{\textwidth}
      \centering
      \includegraphics[height=1.8cm, width=0.8\textwidth]{J0826+2637_2015-11-14_S1_B_BN_dis.ps}
      \caption{\scriptsize Burst and Null lengths}
    \end{subfigure}%
    \vfill
    \begin{subfigure}{\textwidth}
      \centering
      \includegraphics[height=1.8cm, width=0.8\textwidth]{J0826+2637_2015-11-14_S1_B_BN_cor.ps}
      \caption{\scriptsize Brust and Null interaction}
    \end{subfigure}
    \vfill
    \begin{subfigure}{\textwidth}
      \centering
      \includegraphics[height=3.0cm,width=0.7\textwidth]{J0826+2637_2015-11-14_S1_B_BN_period.ps}
      \caption{\scriptsize Nulling periodicity}
    \end{subfigure}
    \vfill
    \begin{subfigure}{\textwidth}
      \centering
      \includegraphics[height=1.7cm,width=0.8\textwidth]{J0826+2637_2015-11-14_S1_B_BE_decay.ps}
      \caption{\scriptsize Variation of burst intensities}
    \end{subfigure}
    \vspace{0pt}% reference point at the very bottom
  \end{minipage}
  \caption{PSR J0826+2637 observed on 2015-11-14 B.}
  \label{fig:J0826_20151114B}
\end{figure}
%%%%%%%%%%%%
\begin{figure}
  \centering
  \sbox{\bigimage}{%
    \begin{subfigure}[b]{.2\textwidth}
      \centering
      \includegraphics[height=1.21cm, width=0.8\textwidth]{J0826+2637_2015-11-15_S1_A_NF_dis.ps}
      \caption{\scriptsize Nulling fraction}
      %\vfill
      \includegraphics[height=7.0cm, width=0.8\textwidth]{J0826+2637_2015-11-15_S1_A_Phase_t.ps}
      \caption{\scriptsize Pulse sequence and states}
      \includegraphics[height=1.0cm,width=0.7\textwidth]{J0826+2637_2015-11-15_S1_A_B_profs.ps}
      \caption{\scriptsize Integrated pulse profiles}
      \vspace{0pt}% reference point at the very bottom
    \end{subfigure}%
  }
  \usebox{\bigimage}
  %\hfill
  \begin{minipage}[b][\ht\bigimage][s]{.2\textwidth}
    \begin{subfigure}{\textwidth}
      \centering
      \includegraphics[height=1.8cm, width=0.8\textwidth]{J0826+2637_2015-11-15_S1_A_BN_dis.ps}
      \caption{\scriptsize Burst and Null lengths}
    \end{subfigure}%
    \vfill
    \begin{subfigure}{\textwidth}
      \centering
      \includegraphics[height=1.8cm, width=0.8\textwidth]{J0826+2637_2015-11-15_S1_A_BN_cor.ps}
      \caption{\scriptsize Brust and Null interaction}
    \end{subfigure}
    \vfill
    \begin{subfigure}{\textwidth}
      \centering
      \includegraphics[height=3.0cm,width=0.7\textwidth]{J0826+2637_2015-11-15_S1_A_BN_period.ps}
      \caption{\scriptsize Nulling periodicity}
    \end{subfigure}
    \vfill
    \begin{subfigure}{\textwidth}
      \centering
      \includegraphics[height=1.7cm,width=0.8\textwidth]{J0826+2637_2015-11-15_S1_A_BE_decay.ps}
      \caption{\scriptsize Variation of burst intensities}
    \end{subfigure}
    \vspace{0pt}% reference point at the very bottom
  \end{minipage}
  \caption{PSR J0826+2637 observed on 2015-11-15 A.}
  \label{fig:J0826_20151115A}
\end{figure}
%%%%%%%%%%%%
\begin{figure}
  \centering
  \sbox{\bigimage}{%
    \begin{subfigure}[b]{.2\textwidth}
      \centering
      \includegraphics[height=1.21cm, width=0.8\textwidth]{J0826+2637_2015-11-15_S1_B_NF_dis.ps}
      \caption{\scriptsize Nulling fraction}
      %\vfill
      \includegraphics[height=7.0cm, width=0.8\textwidth]{J0826+2637_2015-11-15_S1_B_Phase_t.ps}
      \caption{\scriptsize Pulse sequence and states}
      \includegraphics[height=1.0cm,width=0.7\textwidth]{J0826+2637_2015-11-15_S1_B_B_profs.ps}
      \caption{\scriptsize Integrated pulse profiles}
      \vspace{0pt}% reference point at the very bottom
    \end{subfigure}%
  }
  \usebox{\bigimage}
  %\hfill
  \begin{minipage}[b][\ht\bigimage][s]{.2\textwidth}
    \begin{subfigure}{\textwidth}
      \centering
      \includegraphics[height=1.8cm, width=0.8\textwidth]{J0826+2637_2015-11-15_S1_B_BN_dis.ps}
      \caption{\scriptsize Burst and Null lengths}
    \end{subfigure}%
    \vfill
    \begin{subfigure}{\textwidth}
      \centering
      \includegraphics[height=1.8cm, width=0.8\textwidth]{J0826+2637_2015-11-15_S1_B_BN_cor.ps}
      \caption{\scriptsize Brust and Null interaction}
    \end{subfigure}
    \vfill
    \begin{subfigure}{\textwidth}
      \centering
      \includegraphics[height=3.0cm,width=0.7\textwidth]{J0826+2637_2015-11-15_S1_B_BN_period.ps}
      \caption{\scriptsize Nulling periodicity}
    \end{subfigure}
    \vfill
    \begin{subfigure}{\textwidth}
      \centering
      \includegraphics[height=1.7cm,width=0.8\textwidth]{J0826+2637_2015-11-15_S1_B_BE_decay.ps}
      \caption{\scriptsize Variation of burst intensities}
    \end{subfigure}
    \vspace{0pt}% reference point at the very bottom
  \end{minipage}
  \caption{PSR J0826+2637 observed on 2015-11-15 B.}
  \label{fig:J0826_20151115B}
\end{figure}
%%%%%%%%%%%%
\begin{figure}
  \centering
  \sbox{\bigimage}{%
    \begin{subfigure}[b]{.2\textwidth}
      \centering
      \includegraphics[height=1.21cm, width=0.8\textwidth]{J0826+2637_2015-12-07_S1_A_NF_dis.ps}
      \caption{\scriptsize Nulling fraction}
      %\vfill
      \includegraphics[height=7.0cm, width=0.8\textwidth]{J0826+2637_2015-12-07_S1_A_Phase_t.ps}
      \caption{\scriptsize Pulse sequence and states}
      \includegraphics[height=1.0cm,width=0.7\textwidth]{J0826+2637_2015-12-07_S1_A_B_profs.ps}
      \caption{\scriptsize Integrated pulse profiles}
      \vspace{0pt}% reference point at the very bottom
    \end{subfigure}%
  }
  \usebox{\bigimage}
  %\hfill
  \begin{minipage}[b][\ht\bigimage][s]{.2\textwidth}
    \begin{subfigure}{\textwidth}
      \centering
      \includegraphics[height=1.8cm, width=0.8\textwidth]{J0826+2637_2015-12-07_S1_A_BN_dis.ps}
      \caption{\scriptsize Burst and Null lengths}
    \end{subfigure}%
    \vfill
    \begin{subfigure}{\textwidth}
      \centering
      \includegraphics[height=1.8cm, width=0.8\textwidth]{J0826+2637_2015-12-07_S1_A_BN_cor.ps}
      \caption{\scriptsize Brust and Null interaction}
    \end{subfigure}
    \vfill
    \begin{subfigure}{\textwidth}
      \centering
      \includegraphics[height=3.0cm,width=0.7\textwidth]{J0826+2637_2015-12-07_S1_A_BN_period.ps}
      \caption{\scriptsize Nulling periodicity}
    \end{subfigure}
    \vfill
    \begin{subfigure}{\textwidth}
      \centering
      \includegraphics[height=1.7cm,width=0.8\textwidth]{J0826+2637_2015-12-07_S1_A_BE_decay.ps}
      \caption{\scriptsize Variation of burst intensities}
    \end{subfigure}
    \vspace{0pt}% reference point at the very bottom
  \end{minipage}
  \caption{PSR J0826+2637 observed on 2015-12-07 A.}
  \label{fig:J0826_20151207A}
\end{figure}

\begin{figure}
  \centering
  \sbox{\bigimage}{%
    \begin{subfigure}[b]{.2\textwidth}
      \centering
      \includegraphics[height=1.21cm, width=0.8\textwidth]{J0826+2637_2015-12-07_S1_B_NF_dis.ps}
      \caption{\scriptsize Nulling fraction}
      %\vfill
      \includegraphics[height=7.0cm, width=0.8\textwidth]{J0826+2637_2015-12-07_S1_B_Phase_t.ps}
      \caption{\scriptsize Pulse sequence and states}
      \includegraphics[height=1.0cm,width=0.7\textwidth]{J0826+2637_2015-12-07_S1_B_B_profs.ps}
      \caption{\scriptsize Integrated pulse profiles}
      \vspace{0pt}% reference point at the very bottom
    \end{subfigure}%
  }
  \usebox{\bigimage}
  %\hfill
  \begin{minipage}[b][\ht\bigimage][s]{.2\textwidth}
    \begin{subfigure}{\textwidth}
      \centering
      \includegraphics[height=1.8cm, width=0.8\textwidth]{J0826+2637_2015-12-07_S1_B_BN_dis.ps}
      \caption{\scriptsize Burst and Null lengths}
    \end{subfigure}%
    \vfill
    \begin{subfigure}{\textwidth}
      \centering
      \includegraphics[height=1.8cm, width=0.8\textwidth]{J0826+2637_2015-12-07_S1_B_BN_cor.ps}
      \caption{\scriptsize Brust and Null interaction}
    \end{subfigure}
    \vfill
    \begin{subfigure}{\textwidth}
      \centering
      \includegraphics[height=3.0cm,width=0.7\textwidth]{J0826+2637_2015-12-07_S1_B_BN_period.ps}
      \caption{\scriptsize Nulling periodicity}
    \end{subfigure}
    \vfill
    \begin{subfigure}{\textwidth}
      \centering
      \includegraphics[height=1.7cm,width=0.8\textwidth]{J0826+2637_2015-12-07_S1_B_BE_decay.ps}
      \caption{\scriptsize Variation of burst intensities}
    \end{subfigure}
    \vspace{0pt}% reference point at the very bottom
  \end{minipage}
  \caption{PSR J0826+2637 observed on 2015-12-07 B.}
  \label{fig:J0826_20151207B}
\end{figure}

%%%%%%%%%%%%%%%%%%%%%%% J0908
\begin{figure}
  \centering
  \sbox{\bigimage}{%
    \begin{subfigure}[b]{.2\textwidth}
      \centering
      \includegraphics[height=1.21cm, width=0.8\textwidth]{J0908-1739_2016-05-23_S4_0_NF_dis.ps}
      \caption{\scriptsize Nulling fraction}
      %\vfill
      \includegraphics[height=7.0cm, width=0.8\textwidth]{J0908-1739_2016-05-23_S4_0_Phase_t.ps}
      \caption{\scriptsize Pulse sequence and states}
      \includegraphics[height=1.0cm,width=0.7\textwidth]{J0908-1739_2016-05-23_S4_0_B_profs.ps}
      \caption{\scriptsize Integrated pulse profiles}
      \vspace{0pt}% reference point at the very bottom
    \end{subfigure}%
  }
  \usebox{\bigimage}
  %\hfill
  \begin{minipage}[b][\ht\bigimage][s]{.2\textwidth}
    \begin{subfigure}{\textwidth}
      \centering
      \includegraphics[height=1.8cm, width=0.8\textwidth]{J0908-1739_2016-05-23_S4_0_BN_dis.ps}
      \caption{\scriptsize Burst and Null lengths}
    \end{subfigure}%
    \vfill
    \begin{subfigure}{\textwidth}
      \centering
      \includegraphics[height=1.8cm, width=0.8\textwidth]{J0908-1739_2016-05-23_S4_0_BN_cor.ps}
      \caption{\scriptsize Brust and Null interaction}
    \end{subfigure}
    \vfill
    \begin{subfigure}{\textwidth}
      \centering
      \includegraphics[height=3.0cm,width=0.7\textwidth]{J0908-1739_2016-05-23_S4_0_BN_period.ps}
      \caption{\scriptsize Nulling periodicity}
    \end{subfigure}
    \vfill
    \begin{subfigure}{\textwidth}
      \centering
      \includegraphics[height=1.7cm,width=0.8\textwidth]{J0908-1739_2016-05-23_S4_0_BE_decay.ps}
      \caption{\scriptsize Variation of burst intensities}
    \end{subfigure}
    \vspace{0pt}% reference point at the very bottom
  \end{minipage}
  \caption{PSR J0908-1739 observed on 2016-05-23.}
  \label{fig:J0908_20160523}
\end{figure}

%%%%%%%%%%%%%%%%%%%%%%%%%%%%%%%%%%%%%%%%%%%%%%%%%%%%%%%%%%%%%%%%%%%%%%%%%%%%%%%%%%%%%%%%%%%%%%%%% J0922
\begin{figure}
  \centering
  \sbox{\bigimage}{%
    \begin{subfigure}[b]{.2\textwidth}
      \centering
      \includegraphics[height=1.21cm, width=0.8\textwidth]{J0922+0638_2015-07-14_S1_A_NF_dis.ps}
      \caption{\scriptsize Nulling fraction}
      %\vfill
      \includegraphics[height=7.0cm, width=0.8\textwidth]{J0922+0638_2015-07-14_S1_A_Phase_t.ps}
      \caption{\scriptsize Pulse sequence and states}
      \includegraphics[height=1.0cm,width=0.7\textwidth]{J0922+0638_2015-07-14_S1_A_B_profs.ps}
      \caption{\scriptsize Integrated pulse profiles}
      \vspace{0pt}% reference point at the very bottom
    \end{subfigure}%
  }
  \usebox{\bigimage}
  %\hfill
  \begin{minipage}[b][\ht\bigimage][s]{.2\textwidth}
    \begin{subfigure}{\textwidth}
      \centering
      \includegraphics[height=1.8cm, width=0.8\textwidth]{J0922+0638_2015-07-14_S1_A_BN_dis.ps}
      \caption{\scriptsize Burst and Null lengths}
    \end{subfigure}%
    \vfill
    \begin{subfigure}{\textwidth}
      \centering
      \includegraphics[height=1.8cm, width=0.8\textwidth]{J0922+0638_2015-07-14_S1_A_BN_cor.ps}
      \caption{\scriptsize Brust and Null interaction}
    \end{subfigure}
    \vfill
    \begin{subfigure}{\textwidth}
      \centering
      \includegraphics[height=3.0cm,width=0.7\textwidth]{J0922+0638_2015-07-14_S1_A_BN_period.ps}
      \caption{\scriptsize Nulling periodicity}
    \end{subfigure}
    \vfill
    \begin{subfigure}{\textwidth}
      \centering
      \includegraphics[height=1.7cm,width=0.8\textwidth]{J0922+0638_2015-07-14_S1_A_BE_decay.ps}
      \caption{\scriptsize Variation of burst intensities}
    \end{subfigure}
    \vspace{0pt}% reference point at the very bottom
  \end{minipage}
  \caption{PSR J0922+0638 observed on 2015-07-14A.}
  \label{fig:J0922_20150714A}
\end{figure}

\begin{figure}
  \centering
  \sbox{\bigimage}{%
    \begin{subfigure}[b]{.2\textwidth}
      \centering
      \includegraphics[height=1.21cm, width=0.8\textwidth]{J0922+0638_2015-07-14_S4_B_NF_dis.ps}
      \caption{\scriptsize Nulling fraction}
      %\vfill
      \includegraphics[height=7.0cm, width=0.8\textwidth]{J0922+0638_2015-07-14_S4_B_Phase_t.ps}
      \caption{\scriptsize Pulse sequence and states}
      \includegraphics[height=1.0cm,width=0.7\textwidth]{J0922+0638_2015-07-14_S4_B_B_profs.ps}
      \caption{\scriptsize Integrated pulse profiles}
      \vspace{0pt}% reference point at the very bottom
    \end{subfigure}%
  }
  \usebox{\bigimage}
  %\hfill
  \begin{minipage}[b][\ht\bigimage][s]{.2\textwidth}
    \begin{subfigure}{\textwidth}
      \centering
      \includegraphics[height=1.8cm, width=0.8\textwidth]{J0922+0638_2015-07-14_S4_B_BN_dis.ps}
      \caption{\scriptsize Burst and Null lengths}
    \end{subfigure}%
    \vfill
    \begin{subfigure}{\textwidth}
      \centering
      \includegraphics[height=1.8cm, width=0.8\textwidth]{J0922+0638_2015-07-14_S4_B_BN_cor.ps}
      \caption{\scriptsize Brust and Null interaction}
    \end{subfigure}
    \vfill
    \begin{subfigure}{\textwidth}
      \centering
      \includegraphics[height=3.0cm,width=0.7\textwidth]{J0922+0638_2015-07-14_S4_B_BN_period.ps}
      \caption{\scriptsize Nulling periodicity}
    \end{subfigure}
    \vfill
    \begin{subfigure}{\textwidth}
      \centering
      \includegraphics[height=1.7cm,width=0.8\textwidth]{J0922+0638_2015-07-14_S4_B_BE_decay.ps}
      \caption{\scriptsize Variation of burst intensities}
    \end{subfigure}
    \vspace{0pt}% reference point at the very bottom
  \end{minipage}
  \caption{PSR J0922+0638 observed on 2015-07-14B.}
  \label{fig:J0922_20150714B}
\end{figure}
%%%%%%%%%%
\begin{figure}
  \centering
  \sbox{\bigimage}{%
    \begin{subfigure}[b]{.2\textwidth}
      \centering
      \includegraphics[height=1.21cm, width=0.8\textwidth]{J0922+0638_2015-08-17_S1_A_NF_dis.ps}
      \caption{\scriptsize Nulling fraction}
      %\vfill
      \includegraphics[height=7.0cm, width=0.8\textwidth]{J0922+0638_2015-08-17_S1_A_Phase_t.ps}
      \caption{\scriptsize Pulse sequence and states}
      \includegraphics[height=1.0cm,width=0.7\textwidth]{J0922+0638_2015-08-17_S1_A_B_profs.ps}
      \caption{\scriptsize Integrated pulse profiles}
      \vspace{0pt}% reference point at the very bottom
    \end{subfigure}%
  }
  \usebox{\bigimage}
  %\hfill
  \begin{minipage}[b][\ht\bigimage][s]{.2\textwidth}
    \begin{subfigure}{\textwidth}
      \centering
      \includegraphics[height=1.8cm, width=0.8\textwidth]{J0922+0638_2015-08-17_S1_A_BN_dis.ps}
      \caption{\scriptsize Burst and Null lengths}
    \end{subfigure}%
    \vfill
    \begin{subfigure}{\textwidth}
      \centering
      \includegraphics[height=1.8cm, width=0.8\textwidth]{J0922+0638_2015-08-17_S1_A_BN_cor.ps}
      \caption{\scriptsize Brust and Null interaction}
    \end{subfigure}
    \vfill
    \begin{subfigure}{\textwidth}
      \centering
      \includegraphics[height=3.0cm,width=0.7\textwidth]{J0922+0638_2015-08-17_S1_A_BN_period.ps}
      \caption{\scriptsize Nulling periodicity}
    \end{subfigure}
    \vfill
    \begin{subfigure}{\textwidth}
      \centering
      \includegraphics[height=1.7cm,width=0.8\textwidth]{J0922+0638_2015-08-17_S1_A_BE_decay.ps}
      \caption{\scriptsize Variation of burst intensities}
    \end{subfigure}
    \vspace{0pt}% reference point at the very bottom
  \end{minipage}
  \caption{PSR J0922+0638 observed on 2015-08-17.}
  \label{fig:J0922_20150817}
\end{figure}
%%%%%%%%%%
\begin{figure}
  \centering
  \sbox{\bigimage}{%
    \begin{subfigure}[b]{.2\textwidth}
      \centering
      \includegraphics[height=1.21cm, width=0.8\textwidth]{J0922+0638_2015-08-18_S1_A_NF_dis.ps}
      \caption{\scriptsize Nulling fraction}
      %\vfill
      \includegraphics[height=7.0cm, width=0.8\textwidth]{J0922+0638_2015-08-18_S1_A_Phase_t.ps}
      \caption{\scriptsize Pulse sequence and states}
      \includegraphics[height=1.0cm,width=0.7\textwidth]{J0922+0638_2015-08-18_S1_A_B_profs.ps}
      \caption{\scriptsize Integrated pulse profiles}
      \vspace{0pt}% reference point at the very bottom
    \end{subfigure}%
  }
  \usebox{\bigimage}
  %\hfill
  \begin{minipage}[b][\ht\bigimage][s]{.2\textwidth}
    \begin{subfigure}{\textwidth}
      \centering
      \includegraphics[height=1.8cm, width=0.8\textwidth]{J0922+0638_2015-08-18_S1_A_BN_dis.ps}
      \caption{\scriptsize Burst and Null lengths}
    \end{subfigure}%
    \vfill
    \begin{subfigure}{\textwidth}
      \centering
      \includegraphics[height=1.8cm, width=0.8\textwidth]{J0922+0638_2015-08-18_S1_A_BN_cor.ps}
      \caption{\scriptsize Brust and Null interaction}
    \end{subfigure}
    \vfill
    \begin{subfigure}{\textwidth}
      \centering
      \includegraphics[height=3.0cm,width=0.7\textwidth]{J0922+0638_2015-08-18_S1_A_BN_period.ps}
      \caption{\scriptsize Nulling periodicity}
    \end{subfigure}
    \vfill
    \begin{subfigure}{\textwidth}
      \centering
      \includegraphics[height=1.7cm,width=0.8\textwidth]{J0922+0638_2015-08-18_S1_A_BE_decay.ps}
      \caption{\scriptsize Variation of burst intensities}
    \end{subfigure}
    \vspace{0pt}% reference point at the very bottom
  \end{minipage}
  \caption{PSR J0922+0638 observed on 2015-08-18A.}
  \label{fig:J0922_20150818A}
\end{figure}
%%%%%%%%%%
\begin{figure}
  \centering
  \sbox{\bigimage}{%
    \begin{subfigure}[b]{.2\textwidth}
      \centering
      \includegraphics[height=1.21cm, width=0.8\textwidth]{J0922+0638_2015-08-18_S4_B_NF_dis.ps}
      \caption{\scriptsize Nulling fraction}
      %\vfill
      \includegraphics[height=7.0cm, width=0.8\textwidth]{J0922+0638_2015-08-18_S4_B_Phase_t.ps}
      \caption{\scriptsize Pulse sequence and states}
      \includegraphics[height=1.0cm,width=0.7\textwidth]{J0922+0638_2015-08-18_S4_B_B_profs.ps}
      \caption{\scriptsize Integrated pulse profiles}
      \vspace{0pt}% reference point at the very bottom
    \end{subfigure}%
  }
  \usebox{\bigimage}
  %\hfill
  \begin{minipage}[b][\ht\bigimage][s]{.2\textwidth}
    \begin{subfigure}{\textwidth}
      \centering
      \includegraphics[height=1.8cm, width=0.8\textwidth]{J0922+0638_2015-08-18_S4_B_BN_dis.ps}
      \caption{\scriptsize Burst and Null lengths}
    \end{subfigure}%
    \vfill
    \begin{subfigure}{\textwidth}
      \centering
      \includegraphics[height=1.8cm, width=0.8\textwidth]{J0922+0638_2015-08-18_S4_B_BN_cor.ps}
      \caption{\scriptsize Brust and Null interaction}
    \end{subfigure}
    \vfill
    \begin{subfigure}{\textwidth}
      \centering
      \includegraphics[height=3.0cm,width=0.7\textwidth]{J0922+0638_2015-08-18_S4_B_BN_period.ps}
      \caption{\scriptsize Nulling periodicity}
    \end{subfigure}
    \vfill
    \begin{subfigure}{\textwidth}
      \centering
      \includegraphics[height=1.7cm,width=0.8\textwidth]{J0922+0638_2015-08-18_S4_B_BE_decay.ps}
      \caption{\scriptsize Variation of burst intensities}
    \end{subfigure}
    \vspace{0pt}% reference point at the very bottom
  \end{minipage}
  \caption{PSR J0922+0638 observed on 2015-08-18B.}
  \label{fig:J0922_20150818B}
\end{figure}

%%%%%%%%%%%%%%%%%%%%%%%%%%%%%%%%%%%%%%%%%%%%%%%%%%%%%%%%%%%%%%%%%%%%%%%%%%%%%%%%%%%%%%%%%%%%%%% J0953
\begin{figure}
  \centering
  \sbox{\bigimage}{%
    \begin{subfigure}[b]{.2\textwidth}
      \centering
      \includegraphics[height=1.21cm, width=0.8\textwidth]{J0953+0755_2015-12-12_S2_0_NF_dis.ps}
      \caption{\scriptsize Nulling fraction}
      %\vfill
      \includegraphics[height=7.0cm, width=0.8\textwidth]{J0953+0755_2015-12-12_S2_0_Phase_t.ps}
      \caption{\scriptsize Pulse sequence and states}
      \includegraphics[height=1.0cm,width=0.7\textwidth]{J0953+0755_2015-12-12_S2_0_B_profs.ps}
      \caption{\scriptsize Integrated pulse profiles}
      \vspace{0pt}% reference point at the very bottom
    \end{subfigure}%
  }
  \usebox{\bigimage}
  %\hfill
  \begin{minipage}[b][\ht\bigimage][s]{.2\textwidth}
    \begin{subfigure}{\textwidth}
      \centering
      \includegraphics[height=1.8cm, width=0.8\textwidth]{J0953+0755_2015-12-12_S2_0_BN_dis.ps}
      \caption{\scriptsize Burst and Null lengths}
    \end{subfigure}%
    \vfill
    \begin{subfigure}{\textwidth}
      \centering
      \includegraphics[height=1.8cm, width=0.8\textwidth]{J0953+0755_2015-12-12_S2_0_BN_cor.ps}
      \caption{\scriptsize Brust and Null interaction}
    \end{subfigure}
    \vfill
    \begin{subfigure}{\textwidth}
      \centering
      \includegraphics[height=3.0cm,width=0.7\textwidth]{J0953+0755_2015-12-12_S2_0_BN_period.ps}
      \caption{\scriptsize Nulling periodicity}
    \end{subfigure}
    \vfill
    \begin{subfigure}{\textwidth}
      \centering
      \includegraphics[height=1.7cm,width=0.8\textwidth]{J0953+0755_2015-12-12_S2_0_BE_decay.ps}
      \caption{\scriptsize Variation of burst intensities}
    \end{subfigure}
    \vspace{0pt}% reference point at the very bottom
  \end{minipage}
  \caption{PSR J0953+0755 observed on 2015-12-12.}
  \label{fig:J0953_20151212}
\end{figure}

%%%%%%%%%%%%%%%%%%%%%%%%%%%%%%%%%%%%%%%%%%%%%%%%%%%%%%%%%%%%%%%%%%%%%%%%%%%%%%%%%%%%%%%%%%%%%%% J1136
\begin{figure}
  \centering
  \sbox{\bigimage}{%
    \begin{subfigure}[b]{.2\textwidth}
      \centering
      \includegraphics[height=1.21cm, width=0.8\textwidth]{J1136+1551_2015-09-19_S1_0_NF_dis.ps}
      \caption{\scriptsize Nulling fraction}
      %\vfill
      \includegraphics[height=7.0cm, width=0.8\textwidth]{J1136+1551_2015-09-19_S1_0_Phase_t.ps}
      \caption{\scriptsize Pulse sequence and states}
      \includegraphics[height=1.0cm,width=0.7\textwidth]{J1136+1551_2015-09-19_S1_0_B_profs.ps}
      \caption{\scriptsize Integrated pulse profiles}
      \vspace{0pt}% reference point at the very bottom
    \end{subfigure}%
  }
  \usebox{\bigimage}
  %\hfill
  \begin{minipage}[b][\ht\bigimage][s]{.2\textwidth}
    \begin{subfigure}{\textwidth}
      \centering
      \includegraphics[height=1.8cm, width=0.8\textwidth]{J1136+1551_2015-09-19_S1_0_BN_dis.ps}
      \caption{\scriptsize Burst and Null lengths}
    \end{subfigure}%
    \vfill
    \begin{subfigure}{\textwidth}
      \centering
      \includegraphics[height=1.8cm, width=0.8\textwidth]{J1136+1551_2015-09-19_S1_0_BN_cor.ps}
      \caption{\scriptsize Brust and Null interaction}
    \end{subfigure}
    \vfill
    \begin{subfigure}{\textwidth}
      \centering
      \includegraphics[height=3.0cm,width=0.7\textwidth]{J1136+1551_2015-09-19_S1_0_BN_period.ps}
      \caption{\scriptsize Nulling periodicity}
    \end{subfigure}
    \vfill
    \begin{subfigure}{\textwidth}
      \centering
      \includegraphics[height=1.7cm,width=0.8\textwidth]{J1136+1551_2015-09-19_S1_0_BE_decay.ps}
      \caption{\scriptsize Variation of burst intensities}
    \end{subfigure}
    \vspace{0pt}% reference point at the very bottom
  \end{minipage}
  \caption{PSR J1136+1551 observed on 2015-09-19.}
  \label{fig:J1136_20150919}
\end{figure}
%%%%%%%%%%%%
\begin{figure}
  \centering
  \sbox{\bigimage}{%
    \begin{subfigure}[b]{.2\textwidth}
      \centering
      \includegraphics[height=1.21cm, width=0.8\textwidth]{J1136+1551_2017-10-25_S1_A_NF_dis.ps}
      \caption{\scriptsize Nulling fraction}
      %\vfill
      \includegraphics[height=7.0cm, width=0.8\textwidth]{J1136+1551_2017-10-25_S1_A_Phase_t.ps}
      \caption{\scriptsize Pulse sequence and states}
      \includegraphics[height=1.0cm,width=0.7\textwidth]{J1136+1551_2017-10-25_S1_A_B_profs.ps}
      \caption{\scriptsize Integrated pulse profiles}
      \vspace{0pt}% reference point at the very bottom
    \end{subfigure}%
  }
  \usebox{\bigimage}
  %\hfill
  \begin{minipage}[b][\ht\bigimage][s]{.2\textwidth}
    \begin{subfigure}{\textwidth}
      \centering
      \includegraphics[height=1.8cm, width=0.8\textwidth]{J1136+1551_2017-10-25_S1_A_BN_dis.ps}
      \caption{\scriptsize Burst and Null lengths}
    \end{subfigure}%
    \vfill
    \begin{subfigure}{\textwidth}
      \centering
      \includegraphics[height=1.8cm, width=0.8\textwidth]{J1136+1551_2017-10-25_S1_A_BN_cor.ps}
      \caption{\scriptsize Brust and Null interaction}
    \end{subfigure}
    \vfill
    \begin{subfigure}{\textwidth}
      \centering
      \includegraphics[height=3.0cm,width=0.7\textwidth]{J1136+1551_2017-10-25_S1_A_BN_period.ps}
      \caption{\scriptsize Nulling periodicity}
    \end{subfigure}
    \vfill
    \begin{subfigure}{\textwidth}
      \centering
      \includegraphics[height=1.7cm,width=0.8\textwidth]{J1136+1551_2017-10-25_S1_A_BE_decay.ps}
      \caption{\scriptsize Variation of burst intensities}
    \end{subfigure}
    \vspace{0pt}% reference point at the very bottom
  \end{minipage}
  \caption{PSR J1136+1551 observed on 2017-10-25A.}
  \label{fig:J1136_20171025A}
\end{figure}
%%%%%%%%%%%%
\begin{figure}
  \centering
  \sbox{\bigimage}{%
    \begin{subfigure}[b]{.2\textwidth}
      \centering
      \includegraphics[height=1.21cm, width=0.8\textwidth]{J1136+1551_2017-10-25_S1_B_NF_dis.ps}
      \caption{\scriptsize Nulling fraction}
      %\vfill
      \includegraphics[height=7.0cm, width=0.8\textwidth]{J1136+1551_2017-10-25_S1_B_Phase_t.ps}
      \caption{\scriptsize Pulse sequence and states}
      \includegraphics[height=1.0cm,width=0.7\textwidth]{J1136+1551_2017-10-25_S1_B_B_profs.ps}
      \caption{\scriptsize Integrated pulse profiles}
      \vspace{0pt}% reference point at the very bottom
    \end{subfigure}%
  }
  \usebox{\bigimage}
  %\hfill
  \begin{minipage}[b][\ht\bigimage][s]{.2\textwidth}
    \begin{subfigure}{\textwidth}
      \centering
      \includegraphics[height=1.8cm, width=0.8\textwidth]{J1136+1551_2017-10-25_S1_B_BN_dis.ps}
      \caption{\scriptsize Burst and Null lengths}
    \end{subfigure}%
    \vfill
    \begin{subfigure}{\textwidth}
      \centering
      \includegraphics[height=1.8cm, width=0.8\textwidth]{J1136+1551_2017-10-25_S1_B_BN_cor.ps}
      \caption{\scriptsize Brust and Null interaction}
    \end{subfigure}
    \vfill
    \begin{subfigure}{\textwidth}
      \centering
      \includegraphics[height=3.0cm,width=0.7\textwidth]{J1136+1551_2017-10-25_S1_B_BN_period.ps}
      \caption{\scriptsize Nulling periodicity}
    \end{subfigure}
    \vfill
    \begin{subfigure}{\textwidth}
      \centering
      \includegraphics[height=1.7cm,width=0.8\textwidth]{J1136+1551_2017-10-25_S1_B_BE_decay.ps}
      \caption{\scriptsize Variation of burst intensities}
    \end{subfigure}
    \vspace{0pt}% reference point at the very bottom
  \end{minipage}
  \caption{PSR J1136+1551 observed on 2017-10-25B.}
  \label{fig:J1136_20171025B}
\end{figure}
%%%%%%%%%%%%
\begin{figure}
  \centering
  \sbox{\bigimage}{%
    \begin{subfigure}[b]{.2\textwidth}
      \centering
      \includegraphics[height=1.21cm, width=0.8\textwidth]{J1136+1551_2017-10-25_S1_C_NF_dis.ps}
      \caption{\scriptsize Nulling fraction}
      %\vfill
      \includegraphics[height=7.0cm, width=0.8\textwidth]{J1136+1551_2017-10-25_S1_C_Phase_t.ps}
      \caption{\scriptsize Pulse sequence and states}
      \includegraphics[height=1.0cm,width=0.7\textwidth]{J1136+1551_2017-10-25_S1_C_B_profs.ps}
      \caption{\scriptsize Integrated pulse profiles}
      \vspace{0pt}% reference point at the very bottom
    \end{subfigure}%
  }
  \usebox{\bigimage}
  %\hfill
  \begin{minipage}[b][\ht\bigimage][s]{.2\textwidth}
    \begin{subfigure}{\textwidth}
      \centering
      \includegraphics[height=1.8cm, width=0.8\textwidth]{J1136+1551_2017-10-25_S1_C_BN_dis.ps}
      \caption{\scriptsize Burst and Null lengths}
    \end{subfigure}%
    \vfill
    \begin{subfigure}{\textwidth}
      \centering
      \includegraphics[height=1.8cm, width=0.8\textwidth]{J1136+1551_2017-10-25_S1_C_BN_cor.ps}
      \caption{\scriptsize Brust and Null interaction}
    \end{subfigure}
    \vfill
    \begin{subfigure}{\textwidth}
      \centering
      \includegraphics[height=3.0cm,width=0.7\textwidth]{J1136+1551_2017-10-25_S1_C_BN_period.ps}
      \caption{\scriptsize Nulling periodicity}
    \end{subfigure}
    \vfill
    \begin{subfigure}{\textwidth}
      \centering
      \includegraphics[height=1.7cm,width=0.8\textwidth]{J1136+1551_2017-10-25_S1_C_BE_decay.ps}
      \caption{\scriptsize Variation of burst intensities}
    \end{subfigure}
    \vspace{0pt}% reference point at the very bottom
  \end{minipage}
  \caption{PSR J1136+1551 observed on 2017-10-25C.}
  \label{fig:J1136_20171025C}
\end{figure}
%%%%%%%%%%%%
\clearpage
%%%%%%%%%%%%
\begin{figure}
  \centering
  \sbox{\bigimage}{%
    \begin{subfigure}[b]{.2\textwidth}
      \centering
      \includegraphics[height=1.21cm, width=0.8\textwidth]{J1136+1551_2017-10-25_S1_D_NF_dis.ps}
      \caption{\scriptsize Nulling fraction}
      %\vfill
      \includegraphics[height=7.0cm, width=0.8\textwidth]{J1136+1551_2017-10-25_S1_D_Phase_t.ps}
      \caption{\scriptsize Pulse sequence and states}
      \includegraphics[height=1.0cm,width=0.7\textwidth]{J1136+1551_2017-10-25_S1_D_B_profs.ps}
      \caption{\scriptsize Integrated pulse profiles}
      \vspace{0pt}% reference point at the very bottom
    \end{subfigure}%
  }
  \usebox{\bigimage}
  %\hfill
  \begin{minipage}[b][\ht\bigimage][s]{.2\textwidth}
    \begin{subfigure}{\textwidth}
      \centering
      \includegraphics[height=1.8cm, width=0.8\textwidth]{J1136+1551_2017-10-25_S1_D_BN_dis.ps}
      \caption{\scriptsize Burst and Null lengths}
    \end{subfigure}%
    \vfill
    \begin{subfigure}{\textwidth}
      \centering
      \includegraphics[height=1.8cm, width=0.8\textwidth]{J1136+1551_2017-10-25_S1_D_BN_cor.ps}
      \caption{\scriptsize Brust and Null interaction}
    \end{subfigure}
    \vfill
    \begin{subfigure}{\textwidth}
      \centering
      \includegraphics[height=3.0cm,width=0.7\textwidth]{J1136+1551_2017-10-25_S1_D_BN_period.ps}
      \caption{\scriptsize Nulling periodicity}
    \end{subfigure}
    \vfill
    \begin{subfigure}{\textwidth}
      \centering
      \includegraphics[height=1.7cm,width=0.8\textwidth]{J1136+1551_2017-10-25_S1_D_BE_decay.ps}
      \caption{\scriptsize Variation of burst intensities}
    \end{subfigure}
    \vspace{0pt}% reference point at the very bottom
  \end{minipage}
  \caption{PSR J1136+1551 observed on 2017-10-25D.}
  \label{fig:J1136_20171025D}
\end{figure}
%%%%%%%%%%%%
\begin{figure}
  \centering
  \sbox{\bigimage}{%
    \begin{subfigure}[b]{.2\textwidth}
      \centering
      \includegraphics[height=1.21cm, width=0.8\textwidth]{J1136+1551_2018-09-16_S1_0_NF_dis.ps}
      \caption{\scriptsize Nulling fraction}
      %\vfill
      \includegraphics[height=7.0cm, width=0.8\textwidth]{J1136+1551_2018-09-16_S1_0_Phase_t.ps}
      \caption{\scriptsize Pulse sequence and states}
      \includegraphics[height=1.0cm,width=0.7\textwidth]{J1136+1551_2018-09-16_S1_0_B_profs.ps}
      \caption{\scriptsize Integrated pulse profiles}
      \vspace{0pt}% reference point at the very bottom
    \end{subfigure}%
  }
  \usebox{\bigimage}
  %\hfill
  \begin{minipage}[b][\ht\bigimage][s]{.2\textwidth}
    \begin{subfigure}{\textwidth}
      \centering
      \includegraphics[height=1.8cm, width=0.8\textwidth]{J1136+1551_2018-09-16_S1_0_BN_dis.ps}
      \caption{\scriptsize Burst and Null lengths}
    \end{subfigure}%
    \vfill
    \begin{subfigure}{\textwidth}
      \centering
      \includegraphics[height=1.8cm, width=0.8\textwidth]{J1136+1551_2018-09-16_S1_0_BN_cor.ps}
      \caption{\scriptsize Brust and Null interaction}
    \end{subfigure}
    \vfill
    \begin{subfigure}{\textwidth}
      \centering
      \includegraphics[height=3.0cm,width=0.7\textwidth]{J1136+1551_2018-09-16_S1_0_BN_period.ps}
      \caption{\scriptsize Nulling periodicity}
    \end{subfigure}
    \vfill
    \begin{subfigure}{\textwidth}
      \centering
      \includegraphics[height=1.7cm,width=0.8\textwidth]{J1136+1551_2018-09-16_S1_0_BE_decay.ps}
      \caption{\scriptsize Variation of burst intensities}
    \end{subfigure}
    \vspace{0pt}% reference point at the very bottom
  \end{minipage}
  \caption{PSR J1136+1551 observed on 2018-09-16.}
  \label{fig:J1136_20180916}
\end{figure}
%%%%%%%%%%%%
\begin{figure}
  \centering
  \sbox{\bigimage}{%
    \begin{subfigure}[b]{.2\textwidth}
      \centering
      \includegraphics[height=1.21cm, width=0.8\textwidth]{J1136+1551_2018-09-28_S1_A_NF_dis.ps}
      \caption{\scriptsize Nulling fraction}
      %\vfill
      \includegraphics[height=7.0cm, width=0.8\textwidth]{J1136+1551_2018-09-28_S1_A_Phase_t.ps}
      \caption{\scriptsize Pulse sequence and states}
      \includegraphics[height=1.0cm,width=0.7\textwidth]{J1136+1551_2018-09-28_S1_A_B_profs.ps}
      \caption{\scriptsize Integrated pulse profiles}
      \vspace{0pt}% reference point at the very bottom
    \end{subfigure}%
  }
  \usebox{\bigimage}
  %\hfill
  \begin{minipage}[b][\ht\bigimage][s]{.2\textwidth}
    \begin{subfigure}{\textwidth}
      \centering
      \includegraphics[height=1.8cm, width=0.8\textwidth]{J1136+1551_2018-09-28_S1_A_BN_dis.ps}
      \caption{\scriptsize Burst and Null lengths}
    \end{subfigure}%
    \vfill
    \begin{subfigure}{\textwidth}
      \centering
      \includegraphics[height=1.8cm, width=0.8\textwidth]{J1136+1551_2018-09-28_S1_A_BN_cor.ps}
      \caption{\scriptsize Brust and Null interaction}
    \end{subfigure}
    \vfill
    \begin{subfigure}{\textwidth}
      \centering
      \includegraphics[height=3.0cm,width=0.7\textwidth]{J1136+1551_2018-09-28_S1_A_BN_period.ps}
      \caption{\scriptsize Nulling periodicity}
    \end{subfigure}
    \vfill
    \begin{subfigure}{\textwidth}
      \centering
      \includegraphics[height=1.7cm,width=0.8\textwidth]{J1136+1551_2018-09-28_S1_A_BE_decay.ps}
      \caption{\scriptsize Variation of burst intensities}
    \end{subfigure}
    \vspace{0pt}% reference point at the very bottom
  \end{minipage}
  \caption{PSR J1136+1551 observed on 2018-09-28A.}
  \label{fig:J1136_20180928A}
\end{figure}
%%%%%%%%%%%%
\begin{figure}
  \centering
  \sbox{\bigimage}{%
    \begin{subfigure}[b]{.2\textwidth}
      \centering
      \includegraphics[height=1.21cm, width=0.8\textwidth]{J1136+1551_2018-09-28_S1_B_NF_dis.ps}
      \caption{\scriptsize Nulling fraction}
      %\vfill
      \includegraphics[height=7.0cm, width=0.8\textwidth]{J1136+1551_2018-09-28_S1_B_Phase_t.ps}
      \caption{\scriptsize Pulse sequence and states}
      \includegraphics[height=1.0cm,width=0.7\textwidth]{J1136+1551_2018-09-28_S1_B_B_profs.ps}
      \caption{\scriptsize Integrated pulse profiles}
      \vspace{0pt}% reference point at the very bottom
    \end{subfigure}%
  }
  \usebox{\bigimage}
  %\hfill
  \begin{minipage}[b][\ht\bigimage][s]{.2\textwidth}
    \begin{subfigure}{\textwidth}
      \centering
      \includegraphics[height=1.8cm, width=0.8\textwidth]{J1136+1551_2018-09-28_S1_B_BN_dis.ps}
      \caption{\scriptsize Burst and Null lengths}
    \end{subfigure}%
    \vfill
    \begin{subfigure}{\textwidth}
      \centering
      \includegraphics[height=1.8cm, width=0.8\textwidth]{J1136+1551_2018-09-28_S1_B_BN_cor.ps}
      \caption{\scriptsize Brust and Null interaction}
    \end{subfigure}
    \vfill
    \begin{subfigure}{\textwidth}
      \centering
      \includegraphics[height=3.0cm,width=0.7\textwidth]{J1136+1551_2018-09-28_S1_B_BN_period.ps}
      \caption{\scriptsize Nulling periodicity}
    \end{subfigure}
    \vfill
    \begin{subfigure}{\textwidth}
      \centering
      \includegraphics[height=1.7cm,width=0.8\textwidth]{J1136+1551_2018-09-28_S1_B_BE_decay.ps}
      \caption{\scriptsize Variation of burst intensities}
    \end{subfigure}
    \vspace{0pt}% reference point at the very bottom
  \end{minipage}
  \caption{PSR J1136+1551 observed on 2018-09-28B.}
  \label{fig:J1136_20180928B}
\end{figure}

%%%%%%%%%%%%%%%%%%%%%%%%%%%%%%%%%%%%%%%%%%%%%%%%%%%%%%%%%%%%%%%%%%%%%%%%%%%%%%%%%%%%%%%%%%%%%%% J1237
\begin{figure}
  \centering
  \sbox{\bigimage}{%
    \begin{subfigure}[b]{.2\textwidth}
      \centering
      \includegraphics[height=1.21cm, width=0.8\textwidth]{J1239+2453_2015-12-12_S1_A_NF_dis.ps}
      \caption{\scriptsize Nulling fraction}
      %\vfill
      \includegraphics[height=7.0cm, width=0.8\textwidth]{J1239+2453_2015-12-12_S1_A_Phase_t.ps}
      \caption{\scriptsize Pulse sequence and states}
      \includegraphics[height=1.0cm,width=0.7\textwidth]{J1239+2453_2015-12-12_S1_A_B_profs.ps}
      \caption{\scriptsize Integrated pulse profiles}
      \vspace{0pt}% reference point at the very bottom
    \end{subfigure}%
  }
  \usebox{\bigimage}
  %\hfill
  \begin{minipage}[b][\ht\bigimage][s]{.2\textwidth}
    \begin{subfigure}{\textwidth}
      \centering
      \includegraphics[height=1.8cm, width=0.8\textwidth]{J1239+2453_2015-12-12_S1_A_BN_dis.ps}
      \caption{\scriptsize Burst and Null lengths}
    \end{subfigure}%
    \vfill
    \begin{subfigure}{\textwidth}
      \centering
      \includegraphics[height=1.8cm, width=0.8\textwidth]{J1239+2453_2015-12-12_S1_A_BN_cor.ps}
      \caption{\scriptsize Brust and Null interaction}
    \end{subfigure}
    \vfill
    \begin{subfigure}{\textwidth}
      \centering
      \includegraphics[height=3.0cm,width=0.7\textwidth]{J1239+2453_2015-12-12_S1_A_BN_period.ps}
      \caption{\scriptsize Nulling periodicity}
    \end{subfigure}
    \vfill
    \begin{subfigure}{\textwidth}
      \centering
      \includegraphics[height=1.7cm,width=0.8\textwidth]{J1239+2453_2015-12-12_S1_A_BE_decay.ps}
      \caption{\scriptsize Variation of burst intensities}
    \end{subfigure}
    \vspace{0pt}% reference point at the very bottom
  \end{minipage}
  \caption{PSR J1239+2453 observed on 2015-12-12A.}
  \label{fig:J1239_20151212A}
\end{figure}
%%%%%%%%%%%%
\begin{figure}
  \centering
  \sbox{\bigimage}{%
    \begin{subfigure}[b]{.2\textwidth}
      \centering
      \includegraphics[height=1.21cm, width=0.8\textwidth]{J1239+2453_2015-12-12_S2_B_NF_dis.ps}
      \caption{\scriptsize Nulling fraction}
      %\vfill
      \includegraphics[height=7.0cm, width=0.8\textwidth]{J1239+2453_2015-12-12_S2_B_Phase_t.ps}
      \caption{\scriptsize Pulse sequence and states}
      \includegraphics[height=1.0cm,width=0.7\textwidth]{J1239+2453_2015-12-12_S2_B_B_profs.ps}
      \caption{\scriptsize Integrated pulse profiles}
      \vspace{0pt}% reference point at the very bottom
    \end{subfigure}%
  }
  \usebox{\bigimage}
  %\hfill
  \begin{minipage}[b][\ht\bigimage][s]{.2\textwidth}
    \begin{subfigure}{\textwidth}
      \centering
      \includegraphics[height=1.8cm, width=0.8\textwidth]{J1239+2453_2015-12-12_S2_B_BN_dis.ps}
      \caption{\scriptsize Burst and Null lengths}
    \end{subfigure}%
    \vfill
    \begin{subfigure}{\textwidth}
      \centering
      \includegraphics[height=1.8cm, width=0.8\textwidth]{J1239+2453_2015-12-12_S2_B_BN_cor.ps}
      \caption{\scriptsize Brust and Null interaction}
    \end{subfigure}
    \vfill
    \begin{subfigure}{\textwidth}
      \centering
      \includegraphics[height=3.0cm,width=0.7\textwidth]{J1239+2453_2015-12-12_S2_B_BN_period.ps}
      \caption{\scriptsize Nulling periodicity}
    \end{subfigure}
    \vfill
    \begin{subfigure}{\textwidth}
      \centering
      \includegraphics[height=1.7cm,width=0.8\textwidth]{J1239+2453_2015-12-12_S2_B_BE_decay.ps}
      \caption{\scriptsize Variation of burst intensities}
    \end{subfigure}
    \vspace{0pt}% reference point at the very bottom
  \end{minipage}
  \caption{PSR J1239+2453 observed on 2015-12-12B.}
  \label{fig:J1239_20151212B}
\end{figure}
%%%%%%%%%%%%
\begin{figure}
  \centering
  \sbox{\bigimage}{%
    \begin{subfigure}[b]{.2\textwidth}
      \centering
      \includegraphics[height=1.21cm, width=0.8\textwidth]{J1239+2453_2015-12-16_S2_A_NF_dis.ps}
      \caption{\scriptsize Nulling fraction}
      %\vfill
      \includegraphics[height=7.0cm, width=0.8\textwidth]{J1239+2453_2015-12-16_S2_A_Phase_t.ps}
      \caption{\scriptsize Pulse sequence and states}
      \includegraphics[height=1.0cm,width=0.7\textwidth]{J1239+2453_2015-12-16_S2_A_B_profs.ps}
      \caption{\scriptsize Integrated pulse profiles}
      \vspace{0pt}% reference point at the very bottom
    \end{subfigure}%
  }
  \usebox{\bigimage}
  %\hfill
  \begin{minipage}[b][\ht\bigimage][s]{.2\textwidth}
    \begin{subfigure}{\textwidth}
      \centering
      \includegraphics[height=1.8cm, width=0.8\textwidth]{J1239+2453_2015-12-16_S2_A_BN_dis.ps}
      \caption{\scriptsize Burst and Null lengths}
    \end{subfigure}%
    \vfill
    \begin{subfigure}{\textwidth}
      \centering
      \includegraphics[height=1.8cm, width=0.8\textwidth]{J1239+2453_2015-12-16_S2_A_BN_cor.ps}
      \caption{\scriptsize Brust and Null interaction}
    \end{subfigure}
    \vfill
    \begin{subfigure}{\textwidth}
      \centering
      \includegraphics[height=3.0cm,width=0.7\textwidth]{J1239+2453_2015-12-16_S2_A_BN_period.ps}
      \caption{\scriptsize Nulling periodicity}
    \end{subfigure}
    \vfill
    \begin{subfigure}{\textwidth}
      \centering
      \includegraphics[height=1.7cm,width=0.8\textwidth]{J1239+2453_2015-12-16_S2_A_BE_decay.ps}
      \caption{\scriptsize Variation of burst intensities}
    \end{subfigure}
    \vspace{0pt}% reference point at the very bottom
  \end{minipage}
  \caption{PSR J1239+2453 observed on 2015-12-16A.}
  \label{fig:J1239_20151216A}
\end{figure}
%%%%%%%%%%%%
\begin{figure}
  \centering
  \sbox{\bigimage}{%
    \begin{subfigure}[b]{.2\textwidth}
      \centering
      \includegraphics[height=1.21cm, width=0.8\textwidth]{J1239+2453_2015-12-16_S1_B_NF_dis.ps}
      \caption{\scriptsize Nulling fraction}
      %\vfill
      \includegraphics[height=7.0cm, width=0.8\textwidth]{J1239+2453_2015-12-16_S1_B_Phase_t.ps}
      \caption{\scriptsize Pulse sequence and states}
      \includegraphics[height=1.0cm,width=0.7\textwidth]{J1239+2453_2015-12-16_S1_B_B_profs.ps}
      \caption{\scriptsize Integrated pulse profiles}
      \vspace{0pt}% reference point at the very bottom
    \end{subfigure}%
  }
  \usebox{\bigimage}
  %\hfill
  \begin{minipage}[b][\ht\bigimage][s]{.2\textwidth}
    \begin{subfigure}{\textwidth}
      \centering
      \includegraphics[height=1.8cm, width=0.8\textwidth]{J1239+2453_2015-12-16_S1_B_BN_dis.ps}
      \caption{\scriptsize Burst and Null lengths}
    \end{subfigure}%
    \vfill
    \begin{subfigure}{\textwidth}
      \centering
      \includegraphics[height=1.8cm, width=0.8\textwidth]{J1239+2453_2015-12-16_S1_B_BN_cor.ps}
      \caption{\scriptsize Brust and Null interaction}
    \end{subfigure}
    \vfill
    \begin{subfigure}{\textwidth}
      \centering
      \includegraphics[height=3.0cm,width=0.7\textwidth]{J1239+2453_2015-12-16_S1_B_BN_period.ps}
      \caption{\scriptsize Nulling periodicity}
    \end{subfigure}
    \vfill
    \begin{subfigure}{\textwidth}
      \centering
      \includegraphics[height=1.7cm,width=0.8\textwidth]{J1239+2453_2015-12-16_S1_B_BE_decay.ps}
      \caption{\scriptsize Variation of burst intensities}
    \end{subfigure}
    \vspace{0pt}% reference point at the very bottom
  \end{minipage}
  \caption{PSR J1239+2453 observed on 2015-12-16B.}
  \label{fig:J1239_20151216B}
\end{figure}
%%%%%%%%%%%%
\begin{figure}
  \centering
  \sbox{\bigimage}{%
    \begin{subfigure}[b]{.2\textwidth}
      \centering
      \includegraphics[height=1.21cm, width=0.8\textwidth]{J1239+2453_2015-12-19_S1_A_NF_dis.ps}
      \caption{\scriptsize Nulling fraction}
      %\vfill
      \includegraphics[height=7.0cm, width=0.8\textwidth]{J1239+2453_2015-12-19_S1_A_Phase_t.ps}
      \caption{\scriptsize Pulse sequence and states}
      \includegraphics[height=1.0cm,width=0.7\textwidth]{J1239+2453_2015-12-19_S1_A_B_profs.ps}
      \caption{\scriptsize Integrated pulse profiles}
      \vspace{0pt}% reference point at the very bottom
    \end{subfigure}%
  }
  \usebox{\bigimage}
  %\hfill
  \begin{minipage}[b][\ht\bigimage][s]{.2\textwidth}
    \begin{subfigure}{\textwidth}
      \centering
      \includegraphics[height=1.8cm, width=0.8\textwidth]{J1239+2453_2015-12-19_S1_A_BN_dis.ps}
      \caption{\scriptsize Burst and Null lengths}
    \end{subfigure}%
    \vfill
    \begin{subfigure}{\textwidth}
      \centering
      \includegraphics[height=1.8cm, width=0.8\textwidth]{J1239+2453_2015-12-19_S1_A_BN_cor.ps}
      \caption{\scriptsize Brust and Null interaction}
    \end{subfigure}
    \vfill
    \begin{subfigure}{\textwidth}
      \centering
      \includegraphics[height=3.0cm,width=0.7\textwidth]{J1239+2453_2015-12-19_S1_A_BN_period.ps}
      \caption{\scriptsize Nulling periodicity}
    \end{subfigure}
    \vfill
    \begin{subfigure}{\textwidth}
      \centering
      \includegraphics[height=1.7cm,width=0.8\textwidth]{J1239+2453_2015-12-19_S1_A_BE_decay.ps}
      \caption{\scriptsize Variation of burst intensities}
    \end{subfigure}
    \vspace{0pt}% reference point at the very bottom
  \end{minipage}
  \caption{PSR J1239+2453 observed on 2015-12-19.}
  \label{fig:J1239_20151219}
\end{figure}
%%%%%%%%%%%%
\begin{figure}
  \centering
  \sbox{\bigimage}{%
    \begin{subfigure}[b]{.2\textwidth}
      \centering
      \includegraphics[height=1.21cm, width=0.8\textwidth]{J1239+2453_2016-02-18_S1_0_NF_dis.ps}
      \caption{\scriptsize Nulling fraction}
      %\vfill
      \includegraphics[height=7.0cm, width=0.8\textwidth]{J1239+2453_2016-02-18_S1_0_Phase_t.ps}
      \caption{\scriptsize Pulse sequence and states}
      \includegraphics[height=1.0cm,width=0.7\textwidth]{J1239+2453_2016-02-18_S1_0_B_profs.ps}
      \caption{\scriptsize Integrated pulse profiles}
      \vspace{0pt}% reference point at the very bottom
    \end{subfigure}%
  }
  \usebox{\bigimage}
  %\hfill
  \begin{minipage}[b][\ht\bigimage][s]{.2\textwidth}
    \begin{subfigure}{\textwidth}
      \centering
      \includegraphics[height=1.8cm, width=0.8\textwidth]{J1239+2453_2016-02-18_S1_0_BN_dis.ps}
      \caption{\scriptsize Burst and Null lengths}
    \end{subfigure}%
    \vfill
    \begin{subfigure}{\textwidth}
      \centering
      \includegraphics[height=1.8cm, width=0.8\textwidth]{J1239+2453_2016-02-18_S1_0_BN_cor.ps}
      \caption{\scriptsize Brust and Null interaction}
    \end{subfigure}
    \vfill
    \begin{subfigure}{\textwidth}
      \centering
      \includegraphics[height=3.0cm,width=0.7\textwidth]{J1239+2453_2016-02-18_S1_0_BN_period.ps}
      \caption{\scriptsize Nulling periodicity}
    \end{subfigure}
    \vfill
    \begin{subfigure}{\textwidth}
      \centering
      \includegraphics[height=1.7cm,width=0.8\textwidth]{J1239+2453_2016-02-18_S1_0_BE_decay.ps}
      \caption{\scriptsize Variation of burst intensities}
    \end{subfigure}
    \vspace{0pt}% reference point at the very bottom
  \end{minipage}
  \caption{PSR J1239+2453 observed on 2016-02-18.}
  \label{fig:J1239_20160218}
\end{figure}
%%%%%%%%%%%%
%%%%%%%%%%%%%%%%%%%%%%%%%%%%%%%%%%%%%%%%%%%%%%%%%%%%%%%%%%%%%%%%%%%%%%%%%%%%%%%%%%%%%%%%%%%%%%% J1509
\begin{figure}
  \centering
  \sbox{\bigimage}{%
    \begin{subfigure}[b]{.2\textwidth}
      \centering
      \includegraphics[height=1.21cm, width=0.8\textwidth]{J1509+5531_2017-10-30_S1_A_NF_dis.ps}
      \caption{\scriptsize Nulling fraction}
      %\vfill
      \includegraphics[height=7.0cm, width=0.8\textwidth]{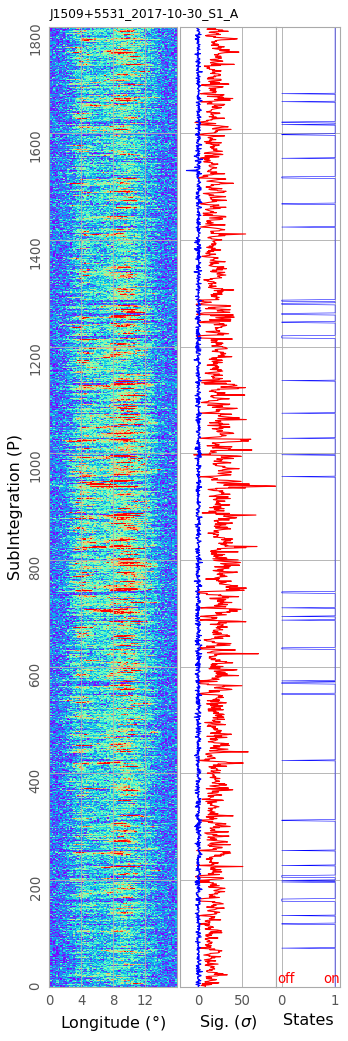}
      \caption{\scriptsize Pulse sequence and states}
      \includegraphics[height=1.0cm,width=0.7\textwidth]{J1509+5531_2017-10-30_S1_A_B_profs.ps}
      \caption{\scriptsize Integrated pulse profiles}
      \vspace{0pt}% reference point at the very bottom
    \end{subfigure}%
  }
  \usebox{\bigimage}
  %\hfill
  \begin{minipage}[b][\ht\bigimage][s]{.2\textwidth}
    \begin{subfigure}{\textwidth}
      \centering
      \includegraphics[height=1.8cm, width=0.8\textwidth]{J1509+5531_2017-10-30_S1_A_BN_dis.ps}
      \caption{\scriptsize Burst and Null lengths}
    \end{subfigure}%
    \vfill
    \begin{subfigure}{\textwidth}
      \centering
      \includegraphics[height=1.8cm, width=0.8\textwidth]{J1509+5531_2017-10-30_S1_A_BN_cor.ps}
      \caption{\scriptsize Brust and Null interaction}
    \end{subfigure}
    \vfill
    \begin{subfigure}{\textwidth}
      \centering
      \includegraphics[height=3.0cm,width=0.7\textwidth]{J1509+5531_2017-10-30_S1_A_BN_period.ps}
      \caption{\scriptsize Nulling periodicity}
    \end{subfigure}
    \vfill
    \begin{subfigure}{\textwidth}
      \centering
      \includegraphics[height=1.7cm,width=0.8\textwidth]{J1509+5531_2017-10-30_S1_A_BE_decay.ps}
      \caption{\scriptsize Variation of burst intensities}
    \end{subfigure}
    \vspace{0pt}% reference point at the very bottom
  \end{minipage}
  \caption{PSR J1509+5531 observed on 2017-10-30A.}
  \label{fig:J1509_20171030A}
\end{figure}
%%%%%%%%%%%%
\begin{figure}
  \centering
  \sbox{\bigimage}{%
    \begin{subfigure}[b]{.2\textwidth}
      \centering
      \includegraphics[height=1.21cm, width=0.8\textwidth]{J1509+5531_2017-10-30_S1_B_NF_dis.ps}
      \caption{\scriptsize Nulling fraction}
      %\vfill
      \includegraphics[height=7.0cm, width=0.8\textwidth]{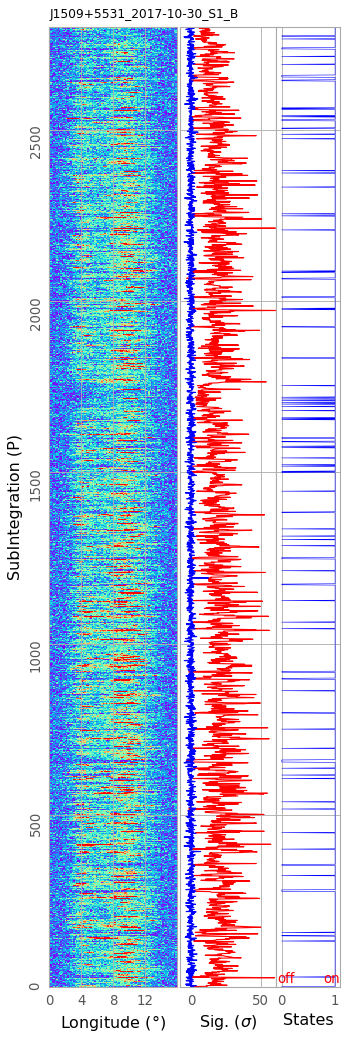}
      \caption{\scriptsize Pulse sequence and states}
      \includegraphics[height=1.0cm,width=0.7\textwidth]{J1509+5531_2017-10-30_S1_B_B_profs.ps}
      \caption{\scriptsize Integrated pulse profiles}
      \vspace{0pt}% reference point at the very bottom
    \end{subfigure}%
  }
  \usebox{\bigimage}
  %\hfill
  \begin{minipage}[b][\ht\bigimage][s]{.2\textwidth}
    \begin{subfigure}{\textwidth}
      \centering
      \includegraphics[height=1.8cm, width=0.8\textwidth]{J1509+5531_2017-10-30_S1_B_BN_dis.ps}
      \caption{\scriptsize Burst and Null lengths}
    \end{subfigure}%
    \vfill
    \begin{subfigure}{\textwidth}
      \centering
      \includegraphics[height=1.8cm, width=0.8\textwidth]{J1509+5531_2017-10-30_S1_B_BN_cor.ps}
      \caption{\scriptsize Brust and Null interaction}
    \end{subfigure}
    \vfill
    \begin{subfigure}{\textwidth}
      \centering
      \includegraphics[height=3.0cm,width=0.7\textwidth]{J1509+5531_2017-10-30_S1_B_BN_period.ps}
      \caption{\scriptsize Nulling periodicity}
    \end{subfigure}
    \vfill
    \begin{subfigure}{\textwidth}
      \centering
      \includegraphics[height=1.7cm,width=0.8\textwidth]{J1509+5531_2017-10-30_S1_B_BE_decay.ps}
      \caption{\scriptsize Variation of burst intensities}
    \end{subfigure}
    \vspace{0pt}% reference point at the very bottom
  \end{minipage}
  \caption{PSR J1509+5531 observed on 2017-10-30B.}
  \label{fig:J1509_20171030B}
\end{figure}
%%%%%%%%%%%%
\begin{figure}
  \centering
  \sbox{\bigimage}{%
    \begin{subfigure}[b]{.2\textwidth}
      \centering
      \includegraphics[height=1.21cm, width=0.8\textwidth]{J1509+5531_2017-10-30_S2_C_NF_dis.ps}
      \caption{\scriptsize Nulling fraction}
      %\vfill
      \includegraphics[height=7.0cm, width=0.8\textwidth]{J1509+5531_2017-10-30_S2_C_Phase_t.ps}
      \caption{\scriptsize Pulse sequence and states}
      \includegraphics[height=1.0cm,width=0.7\textwidth]{J1509+5531_2017-10-30_S2_C_B_profs.ps}
      \caption{\scriptsize Integrated pulse profiles}
      \vspace{0pt}% reference point at the very bottom
    \end{subfigure}%
  }
  \usebox{\bigimage}
  %\hfill
  \begin{minipage}[b][\ht\bigimage][s]{.2\textwidth}
    \begin{subfigure}{\textwidth}
      \centering
      \includegraphics[height=1.8cm, width=0.8\textwidth]{J1509+5531_2017-10-30_S2_C_BN_dis.ps}
      \caption{\scriptsize Burst and Null lengths}
    \end{subfigure}%
    \vfill
    \begin{subfigure}{\textwidth}
      \centering
      \includegraphics[height=1.8cm, width=0.8\textwidth]{J1509+5531_2017-10-30_S2_C_BN_cor.ps}
      \caption{\scriptsize Brust and Null interaction}
    \end{subfigure}
    \vfill
    \begin{subfigure}{\textwidth}
      \centering
      \includegraphics[height=3.0cm,width=0.7\textwidth]{J1509+5531_2017-10-30_S2_C_BN_period.ps}
      \caption{\scriptsize Nulling periodicity}
    \end{subfigure}
    \vfill
    \begin{subfigure}{\textwidth}
      \centering
      \includegraphics[height=1.7cm,width=0.8\textwidth]{J1509+5531_2017-10-30_S2_C_BE_decay.ps}
      \caption{\scriptsize Variation of burst intensities}
    \end{subfigure}
    \vspace{0pt}% reference point at the very bottom
  \end{minipage}
  \caption{PSR J1509+5531 observed on 2017-10-30C.}
  \label{fig:J1509_20171030C}
\end{figure}

%%%%%%%%%%%%
%%%%%%%%%%%%%%%%%%%%%%%%%%%%%%%%%%%%%%%%%%%%%%%%%%%%%%%%%%%%%%%%%%%%%%%%%%%%%%%%%%%%%%%%%%%%%%% J1844
\begin{figure}
  \centering
  \sbox{\bigimage}{%
    \begin{subfigure}[b]{.2\textwidth}
      \centering
      \includegraphics[height=1.21cm, width=0.8\textwidth]{J1844+00_2018-08-09_S16_0_NF_dis.ps}
      \caption{\scriptsize Nulling fraction}
      %\vfill
      \includegraphics[height=7.0cm, width=0.8\textwidth]{J1844+00_2018-08-09_S16_0_Phase_t.ps}
      \caption{\scriptsize Pulse sequence and states}
      \includegraphics[height=1.0cm,width=0.7\textwidth]{J1844+00_2018-08-09_S16_0_B_profs.ps}
      \caption{\scriptsize Integrated pulse profiles}
      \vspace{0pt}% reference point at the very bottom
    \end{subfigure}%
  }
  \usebox{\bigimage}
  %\hfill
  \begin{minipage}[b][\ht\bigimage][s]{.2\textwidth}
    \begin{subfigure}{\textwidth}
      \centering
      \includegraphics[height=1.8cm, width=0.8\textwidth]{J1844+00_2018-08-09_S16_0_BN_dis.ps}
      \caption{\scriptsize Burst and Null lengths}
    \end{subfigure}%
    \vfill
    \begin{subfigure}{\textwidth}
      \centering
      \includegraphics[height=1.8cm, width=0.8\textwidth]{J1844+00_2018-08-09_S16_0_BN_cor.ps}
      \caption{\scriptsize Brust and Null interaction}
    \end{subfigure}
    \vfill
    \begin{subfigure}{\textwidth}
      \centering
      \includegraphics[height=3.0cm,width=0.7\textwidth]{J1844+00_2018-08-09_S16_0_BN_period.ps}
      \caption{\scriptsize Nulling periodicity}
    \end{subfigure}
    \vfill
    \begin{subfigure}{\textwidth}
      \centering
      \includegraphics[height=1.7cm,width=0.8\textwidth]{J1844+00_2018-08-09_S16_0_BE_decay.ps}
      \caption{\scriptsize Variation of burst intensities}
    \end{subfigure}
    \vspace{0pt}% reference point at the very bottom
  \end{minipage}
  \caption{PSR J1844+00 observed on 2018-08-09.}
  \label{fig:J1844_20180809}
\end{figure}
%%%%%%%%%%%%
%%%%%%%%%%%%
\clearpage
%%%%%%%%%%%%
%%%%%%%%%%%%%%%%%%%%%%%%%%%%%%%%%%%%%%%%%%%%%%%%%%%%%%%%%%%%%%%%%%%%%%%%%%%%%%%%%%%%%%%%%%%%%%% J1932
\begin{figure}
  \centering
  \sbox{\bigimage}{%
    \begin{subfigure}[b]{.2\textwidth}
      \centering
      \includegraphics[height=1.21cm, width=0.8\textwidth]{J1932+1059_2016-02-21_S1_A_NF_dis.ps}
      \caption{\scriptsize Nulling fraction}
      %\vfill
      \includegraphics[height=7.0cm, width=0.8\textwidth]{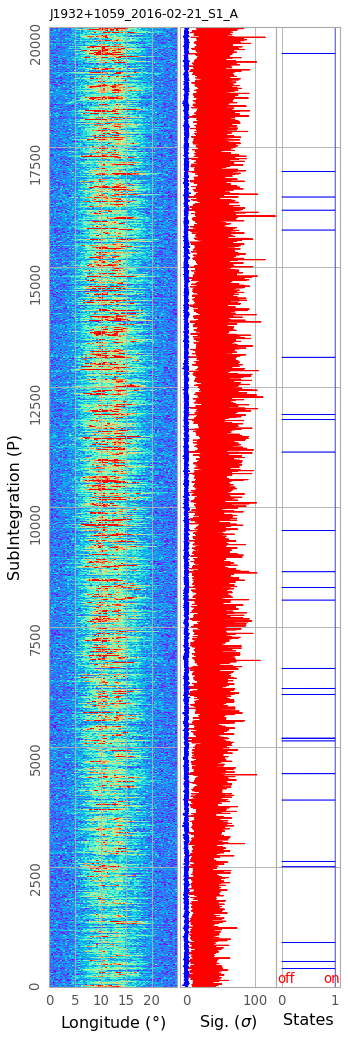}
      \caption{\scriptsize Pulse sequence and states}
      \includegraphics[height=1.0cm,width=0.7\textwidth]{J1932+1059_2016-02-21_S1_A_B_profs.ps}
      \caption{\scriptsize Integrated pulse profiles}
      \vspace{0pt}% reference point at the very bottom
    \end{subfigure}%
  }
  \usebox{\bigimage}
  %\hfill
  \begin{minipage}[b][\ht\bigimage][s]{.2\textwidth}
    \begin{subfigure}{\textwidth}
      \centering
      \includegraphics[height=1.8cm, width=0.8\textwidth]{J1932+1059_2016-02-21_S1_A_BN_dis.ps}
      \caption{\scriptsize Burst and Null lengths}
    \end{subfigure}%
    \vfill
    \begin{subfigure}{\textwidth}
      \centering
      \includegraphics[height=1.8cm, width=0.8\textwidth]{J1932+1059_2016-02-21_S1_A_BN_cor.ps}
      \caption{\scriptsize Brust and Null interaction}
    \end{subfigure}
    \vfill
    \begin{subfigure}{\textwidth}
      \centering
      \includegraphics[height=3.0cm,width=0.7\textwidth]{J1932+1059_2016-02-21_S1_A_BN_period.ps}
      \caption{\scriptsize Nulling periodicity}
    \end{subfigure}
    \vfill
    \begin{subfigure}{\textwidth}
      \centering
      \includegraphics[height=1.7cm,width=0.8\textwidth]{J1932+1059_2016-02-21_S1_A_BE_decay.ps}
      \caption{\scriptsize Variation of burst intensities}
    \end{subfigure}
    \vspace{0pt}% reference point at the very bottom
  \end{minipage}
  \caption{PSR J1932+1059 observed on 2016-02-21A.}
  \label{fig:J1932_20160221A}
\end{figure}
%%%%%%%%%%%%
%%%%%%%%%%%%
\begin{figure}
  \centering
  \sbox{\bigimage}{%
    \begin{subfigure}[b]{.2\textwidth}
      \centering
      \includegraphics[height=1.21cm, width=0.8\textwidth]{J1932+1059_2016-02-21_S1_B_NF_dis.ps}
      \caption{\scriptsize Nulling fraction}
      %\vfill
      \includegraphics[height=7.0cm, width=0.8\textwidth]{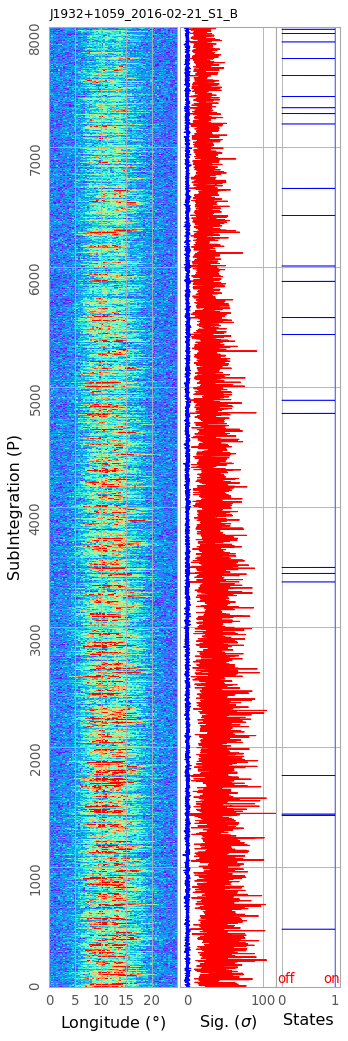}
      \caption{\scriptsize Pulse sequence and states}
      \includegraphics[height=1.0cm,width=0.7\textwidth]{J1932+1059_2016-02-21_S1_B_B_profs.ps}
      \caption{\scriptsize Integrated pulse profiles}
      \vspace{0pt}% reference point at the very bottom
    \end{subfigure}%
  }
  \usebox{\bigimage}
  %\hfill
  \begin{minipage}[b][\ht\bigimage][s]{.2\textwidth}
    \begin{subfigure}{\textwidth}
      \centering
      \includegraphics[height=1.8cm, width=0.8\textwidth]{J1932+1059_2016-02-21_S1_B_BN_dis.ps}
      \caption{\scriptsize Burst and Null lengths}
    \end{subfigure}%
    \vfill
    \begin{subfigure}{\textwidth}
      \centering
      \includegraphics[height=1.8cm, width=0.8\textwidth]{J1932+1059_2016-02-21_S1_B_BN_cor.ps}
      \caption{\scriptsize Brust and Null interaction}
    \end{subfigure}
    \vfill
    \begin{subfigure}{\textwidth}
      \centering
      \includegraphics[height=3.0cm,width=0.7\textwidth]{J1932+1059_2016-02-21_S1_B_BN_period.ps}
      \caption{\scriptsize Nulling periodicity}
    \end{subfigure}
    \vfill
    \begin{subfigure}{\textwidth}
      \centering
      \includegraphics[height=1.7cm,width=0.8\textwidth]{J1932+1059_2016-02-21_S1_B_BE_decay.ps}
      \caption{\scriptsize Variation of burst intensities}
    \end{subfigure}
    \vspace{0pt}% reference point at the very bottom
  \end{minipage}
  \caption{PSR J1932+1059 observed on 2016-02-21B.}
  \label{fig:J1932_20160221B}
\end{figure}
%%%%%%%%%%%%
\begin{figure}
  \centering
  \sbox{\bigimage}{%
    \begin{subfigure}[b]{.2\textwidth}
      \centering
      \includegraphics[height=1.21cm, width=0.8\textwidth]{J1932+1059_2016-02-21_S1_C_NF_dis.ps}
      \caption{\scriptsize Nulling fraction}
      %\vfill
      \includegraphics[height=7.0cm, width=0.8\textwidth]{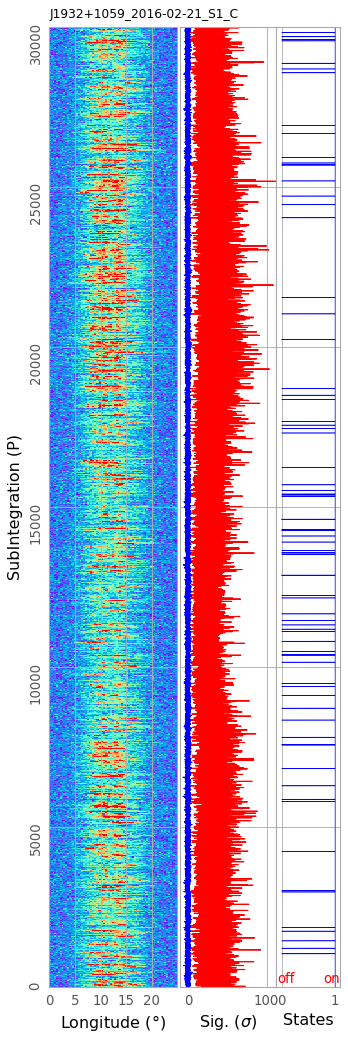}
      \caption{\scriptsize Pulse sequence and states}
      \includegraphics[height=1.0cm,width=0.7\textwidth]{J1932+1059_2016-02-21_S1_C_B_profs.ps}
      \caption{\scriptsize Integrated pulse profiles}
      \vspace{0pt}% reference point at the very bottom
    \end{subfigure}%
  }
  \usebox{\bigimage}
  %\hfill
  \begin{minipage}[b][\ht\bigimage][s]{.2\textwidth}
    \begin{subfigure}{\textwidth}
      \centering
      \includegraphics[height=1.8cm, width=0.8\textwidth]{J1932+1059_2016-02-21_S1_C_BN_dis.ps}
      \caption{\scriptsize Burst and Null lengths}
    \end{subfigure}%
    \vfill
    \begin{subfigure}{\textwidth}
      \centering
      \includegraphics[height=1.8cm, width=0.8\textwidth]{J1932+1059_2016-02-21_S1_C_BN_cor.ps}
      \caption{\scriptsize Brust and Null interaction}
    \end{subfigure}
    \vfill
    \begin{subfigure}{\textwidth}
      \centering
      \includegraphics[height=3.0cm,width=0.7\textwidth]{J1932+1059_2016-02-21_S1_C_BN_period.ps}
      \caption{\scriptsize Nulling periodicity}
    \end{subfigure}
    \vfill
    \begin{subfigure}{\textwidth}
      \centering
      \includegraphics[height=1.7cm,width=0.8\textwidth]{J1932+1059_2016-02-21_S1_C_BE_decay.ps}
      \caption{\scriptsize Variation of burst intensities}
    \end{subfigure}
    \vspace{0pt}% reference point at the very bottom
  \end{minipage}
  \caption{PSR J1932+1059 observed on 2016-02-21C.}
  \label{fig:J1932_20160221C}
\end{figure}
%%%%%%%%%%%%
\begin{figure}
  \centering
  \sbox{\bigimage}{%
    \begin{subfigure}[b]{.2\textwidth}
      \centering
      \includegraphics[height=1.21cm, width=0.8\textwidth]{J1932+1059_2016-02-21_S1_D_NF_dis.ps}
      \caption{\scriptsize Nulling fraction}
      %\vfill
      \includegraphics[height=7.0cm, width=0.8\textwidth]{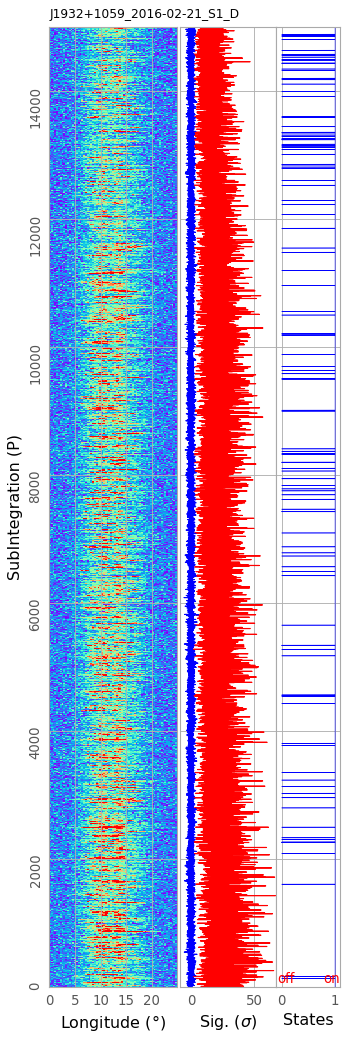}
      \caption{\scriptsize Pulse sequence and states}
      \includegraphics[height=1.0cm,width=0.7\textwidth]{J1932+1059_2016-02-21_S1_D_B_profs.ps}
      \caption{\scriptsize Integrated pulse profiles}
      \vspace{0pt}% reference point at the very bottom
    \end{subfigure}%
  }
  \usebox{\bigimage}
  %\hfill
  \begin{minipage}[b][\ht\bigimage][s]{.2\textwidth}
    \begin{subfigure}{\textwidth}
      \centering
      \includegraphics[height=1.8cm, width=0.8\textwidth]{J1932+1059_2016-02-21_S1_D_BN_dis.ps}
      \caption{\scriptsize Burst and Null lengths}
    \end{subfigure}%
    \vfill
    \begin{subfigure}{\textwidth}
      \centering
      \includegraphics[height=1.8cm, width=0.8\textwidth]{J1932+1059_2016-02-21_S1_D_BN_cor.ps}
      \caption{\scriptsize Brust and Null interaction}
    \end{subfigure}
    \vfill
    \begin{subfigure}{\textwidth}
      \centering
      \includegraphics[height=3.0cm,width=0.7\textwidth]{J1932+1059_2016-02-21_S1_D_BN_period.ps}
      \caption{\scriptsize Nulling periodicity}
    \end{subfigure}
    \vfill
    \begin{subfigure}{\textwidth}
      \centering
      \includegraphics[height=1.7cm,width=0.8\textwidth]{J1932+1059_2016-02-21_S1_D_BE_decay.ps}
      \caption{\scriptsize Variation of burst intensities}
    \end{subfigure}
    \vspace{0pt}% reference point at the very bottom
  \end{minipage}
  \caption{PSR J1932+1059 observed on 2016-02-21D.}
  \label{fig:J1932_20160221D}
\end{figure}

%%%%%%%%%%%%%%%%%%%%%%%%%%%%%%%%%%%%%%%%%%%%%%%%%%%%%%%%%%%%%%%%%%%%%%%%%%%%%%%%%%%%%%%%%%%%%%% J2022
\begin{figure}
  \centering
  \sbox{\bigimage}{%
    \begin{subfigure}[b]{.2\textwidth}
      \centering
      \includegraphics[height=1.21cm, width=0.8\textwidth]{J2022+5154_2015-06-15_S1_0_NF_dis.ps}
      \caption{\scriptsize Nulling fraction}
      %\vfill
      \includegraphics[height=7.0cm, width=0.8\textwidth]{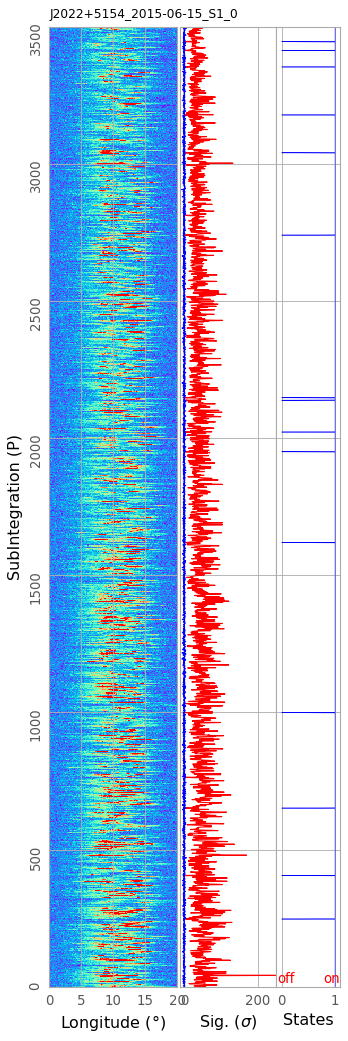}
      \caption{\scriptsize Pulse sequence and states}
      \includegraphics[height=1.0cm,width=0.7\textwidth]{J2022+5154_2015-06-15_S1_0_B_profs.ps}
      \caption{\scriptsize Integrated pulse profiles}
      \vspace{0pt}% reference point at the very bottom
    \end{subfigure}%
  }
  \usebox{\bigimage}
  %\hfill
  \begin{minipage}[b][\ht\bigimage][s]{.2\textwidth}
    \begin{subfigure}{\textwidth}
      \centering
      \includegraphics[height=1.8cm, width=0.8\textwidth]{J2022+5154_2015-06-15_S1_0_BN_dis.ps}
      \caption{\scriptsize Burst and Null lengths}
    \end{subfigure}%
    \vfill
    \begin{subfigure}{\textwidth}
      \centering
      \includegraphics[height=1.8cm, width=0.8\textwidth]{J2022+5154_2015-06-15_S1_0_BN_cor.ps}
      \caption{\scriptsize Brust and Null interaction}
    \end{subfigure}
    \vfill
    \begin{subfigure}{\textwidth}
      \centering
      \includegraphics[height=3.0cm,width=0.7\textwidth]{J2022+5154_2015-06-15_S1_0_BN_period.ps}
      \caption{\scriptsize Nulling periodicity}
    \end{subfigure}
    \vfill
    \begin{subfigure}{\textwidth}
      \centering
      \includegraphics[height=1.7cm,width=0.8\textwidth]{J2022+5154_2015-06-15_S1_0_BE_decay.ps}
      \caption{\scriptsize Variation of burst intensities}
    \end{subfigure}
    \vspace{0pt}% reference point at the very bottom
  \end{minipage}
  \caption{PSR J2022+5154 observed on 2015-06-15.}
  \label{fig:J2022_20150615}
\end{figure}
%%%%%%%%%%%%
\begin{figure}
  \centering
  \sbox{\bigimage}{%
    \begin{subfigure}[b]{.2\textwidth}
      \centering
      \includegraphics[height=1.21cm, width=0.8\textwidth]{J2022+5154_2017-11-01_S1_0_NF_dis.ps}
      \caption{\scriptsize Nulling fraction}
      %\vfill
      \includegraphics[height=7.0cm, width=0.8\textwidth]{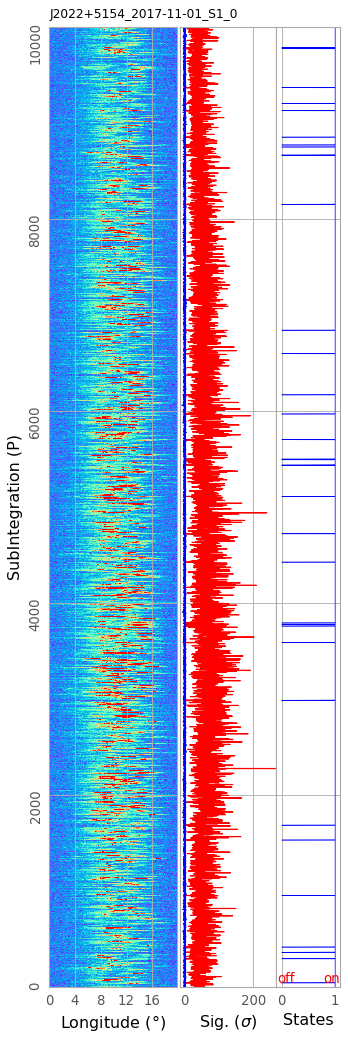}
      \caption{\scriptsize Pulse sequence and states}
      \includegraphics[height=1.0cm,width=0.7\textwidth]{J2022+5154_2017-11-01_S1_0_B_profs.ps}
      \caption{\scriptsize Integrated pulse profiles}
      \vspace{0pt}% reference point at the very bottom
    \end{subfigure}%
  }
  \usebox{\bigimage}
  %\hfill
  \begin{minipage}[b][\ht\bigimage][s]{.2\textwidth}
    \begin{subfigure}{\textwidth}
      \centering
      \includegraphics[height=1.8cm, width=0.8\textwidth]{J2022+5154_2017-11-01_S1_0_BN_dis.ps}
      \caption{\scriptsize Burst and Null lengths}
    \end{subfigure}%
    \vfill
    \begin{subfigure}{\textwidth}
      \centering
      \includegraphics[height=1.8cm, width=0.8\textwidth]{J2022+5154_2017-11-01_S1_0_BN_cor.ps}
      \caption{\scriptsize Brust and Null interaction}
    \end{subfigure}
    \vfill
    \begin{subfigure}{\textwidth}
      \centering
      \includegraphics[height=3.0cm,width=0.7\textwidth]{J2022+5154_2017-11-01_S1_0_BN_period.ps}
      \caption{\scriptsize Nulling periodicity}
    \end{subfigure}
    \vfill
    \begin{subfigure}{\textwidth}
      \centering
      \includegraphics[height=1.7cm,width=0.8\textwidth]{J2022+5154_2017-11-01_S1_0_BE_decay.ps}
      \caption{\scriptsize Variation of burst intensities}
    \end{subfigure}
    \vspace{0pt}% reference point at the very bottom
  \end{minipage}
  \caption{PSR J2022+5154 observed on 2017-11-01.}
  \label{fig:J2022_20171101}
\end{figure}
%%%%%%%%%%%%
\begin{figure}
  \centering
  \sbox{\bigimage}{%
    \begin{subfigure}[b]{.2\textwidth}
      \centering
      \includegraphics[height=1.21cm, width=0.8\textwidth]{J2022+5154_2017-11-06_S1_0_NF_dis.ps}
      \caption{\scriptsize Nulling fraction}
      %\vfill
      \includegraphics[height=7.0cm, width=0.8\textwidth]{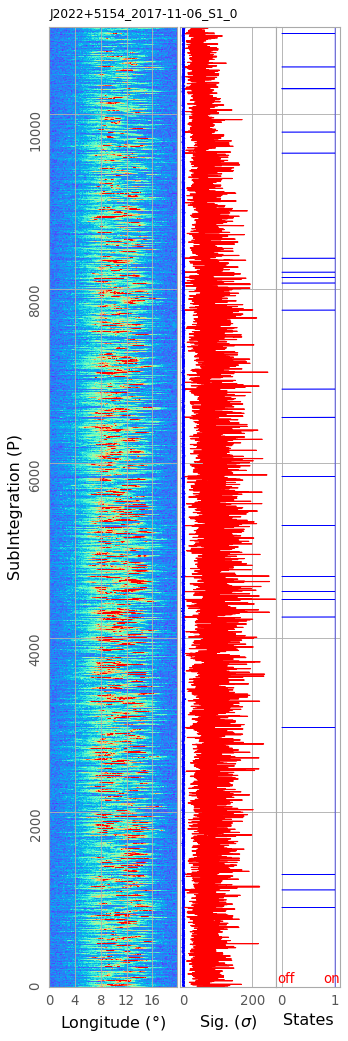}
      \caption{\scriptsize Pulse sequence and states}
      \includegraphics[height=1.0cm,width=0.7\textwidth]{J2022+5154_2017-11-06_S1_0_B_profs.ps}
      \caption{\scriptsize Integrated pulse profiles}
      \vspace{0pt}% reference point at the very bottom
    \end{subfigure}%
  }
  \usebox{\bigimage}
  %\hfill
  \begin{minipage}[b][\ht\bigimage][s]{.2\textwidth}
    \begin{subfigure}{\textwidth}
      \centering
      \includegraphics[height=1.8cm, width=0.8\textwidth]{J2022+5154_2017-11-06_S1_0_BN_dis.ps}
      \caption{\scriptsize Burst and Null lengths}
    \end{subfigure}%
    \vfill
    \begin{subfigure}{\textwidth}
      \centering
      \includegraphics[height=1.8cm, width=0.8\textwidth]{J2022+5154_2017-11-06_S1_0_BN_cor.ps}
      \caption{\scriptsize Brust and Null interaction}
    \end{subfigure}
    \vfill
    \begin{subfigure}{\textwidth}
      \centering
      \includegraphics[height=3.0cm,width=0.7\textwidth]{J2022+5154_2017-11-06_S1_0_BN_period.ps}
      \caption{\scriptsize Nulling periodicity}
    \end{subfigure}
    \vfill
    \begin{subfigure}{\textwidth}
      \centering
      \includegraphics[height=1.7cm,width=0.8\textwidth]{J2022+5154_2017-11-06_S1_0_BE_decay.ps}
      \caption{\scriptsize Variation of burst intensities}
    \end{subfigure}
    \vspace{0pt}% reference point at the very bottom
  \end{minipage}
  \caption{PSR J2022+5154 observed on 2017-11-06.}
  \label{fig:J2022_20171106}
\end{figure}
%%%%%%%%%%%%
%%%%%%%%%%%%%%%%%%%%%%%%%%%%%%%%%%%%%%%%%%%%%%%%%%%%%%%%%%%%%%%%%%%%%%%%%%%%%%%%%%%%%%%%%%%%%%% J2048
\begin{figure}
  \centering
  \sbox{\bigimage}{%
    \begin{subfigure}[b]{.2\textwidth}
      \centering
      \includegraphics[height=1.21cm, width=0.8\textwidth]{J2048-1616_2015-06-18_S1_0_NF_dis.ps}
      \caption{\scriptsize Nulling fraction}
      %\vfill
      \includegraphics[height=7.0cm, width=0.8\textwidth]{J2048-1616_2015-06-18_S1_0_Phase_t.ps}
      \caption{\scriptsize Pulse sequence and states}
      \includegraphics[height=1.0cm,width=0.7\textwidth]{J2048-1616_2015-06-18_S1_0_B_profs.ps}
      \caption{\scriptsize Integrated pulse profiles}
      \vspace{0pt}% reference point at the very bottom
    \end{subfigure}%
  }
  \usebox{\bigimage}
  %\hfill
  \begin{minipage}[b][\ht\bigimage][s]{.2\textwidth}
    \begin{subfigure}{\textwidth}
      \centering
      \includegraphics[height=1.8cm, width=0.8\textwidth]{J2048-1616_2015-06-18_S1_0_BN_dis.ps}
      \caption{\scriptsize Burst and Null lengths}
    \end{subfigure}%
    \vfill
    \begin{subfigure}{\textwidth}
      \centering
      \includegraphics[height=1.8cm, width=0.8\textwidth]{J2048-1616_2015-06-18_S1_0_BN_cor.ps}
      \caption{\scriptsize Brust and Null interaction}
    \end{subfigure}
    \vfill
    \begin{subfigure}{\textwidth}
      \centering
      \includegraphics[height=3.0cm,width=0.7\textwidth]{J2048-1616_2015-06-18_S1_0_BN_period.ps}
      \caption{\scriptsize Nulling periodicity}
    \end{subfigure}
    \vfill
    \begin{subfigure}{\textwidth}
      \centering
      \includegraphics[height=1.7cm,width=0.8\textwidth]{J2048-1616_2015-06-18_S1_0_BE_decay.ps}
      \caption{\scriptsize Variation of burst intensities}
    \end{subfigure}
    \vspace{0pt}% reference point at the very bottom
  \end{minipage}
  \caption{PSR J2048-1616 observed on 2015-06-18.}
  \label{fig:J2048_20150618}
\end{figure}
%%%%%%%%%%%%
\begin{figure}
  \centering
  \sbox{\bigimage}{%
    \begin{subfigure}[b]{.2\textwidth}
      \centering
      \includegraphics[height=1.21cm, width=0.8\textwidth]{J2048-1616_2016-08-08_S1_A_NF_dis.ps}
      \caption{\scriptsize Nulling fraction}
      %\vfill
      \includegraphics[height=7.0cm, width=0.8\textwidth]{J2048-1616_2016-08-08_S1_A_Phase_t.ps}
      \caption{\scriptsize Pulse sequence and states}
      \includegraphics[height=1.0cm,width=0.7\textwidth]{J2048-1616_2016-08-08_S1_A_B_profs.ps}
      \caption{\scriptsize Integrated pulse profiles}
      \vspace{0pt}% reference point at the very bottom
    \end{subfigure}%
  }
  \usebox{\bigimage}
  %\hfill
  \begin{minipage}[b][\ht\bigimage][s]{.2\textwidth}
    \begin{subfigure}{\textwidth}
      \centering
      \includegraphics[height=1.8cm, width=0.8\textwidth]{J2048-1616_2016-08-08_S1_A_BN_dis.ps}
      \caption{\scriptsize Burst and Null lengths}
    \end{subfigure}%
    \vfill
    \begin{subfigure}{\textwidth}
      \centering
      \includegraphics[height=1.8cm, width=0.8\textwidth]{J2048-1616_2016-08-08_S1_A_BN_cor.ps}
      \caption{\scriptsize Brust and Null interaction}
    \end{subfigure}
    \vfill
    \begin{subfigure}{\textwidth}
      \centering
      \includegraphics[height=3.0cm,width=0.7\textwidth]{J2048-1616_2016-08-08_S1_A_BN_period.ps}
      \caption{\scriptsize Nulling periodicity}
    \end{subfigure}
    \vfill
    \begin{subfigure}{\textwidth}
      \centering
      \includegraphics[height=1.7cm,width=0.8\textwidth]{J2048-1616_2016-08-08_S1_A_BE_decay.ps}
      \caption{\scriptsize Variation of burst intensities}
    \end{subfigure}
    \vspace{0pt}% reference point at the very bottom
  \end{minipage}
  \caption{PSR J2048-1616 observed on 2016-08-08.}
  \label{fig:J2048_20160808}
\end{figure}
%%%%%%%%%%%%
%%%%%%%%%%%%%%%%%%%%%%%%%%%%%%%%%%%%%%%%%%%%%%%%%%%%%%%%%%%%%%%%%%%%%%%%%%%%%%%%%%%%%%%%%%%%%%% J2313
\begin{figure}
  \centering
  \sbox{\bigimage}{%
    \begin{subfigure}[b]{.2\textwidth}
      \centering
      \includegraphics[height=1.21cm, width=0.8\textwidth]{J2313+4253_2017-10-25_S1_A_NF_dis.ps}
      \caption{\scriptsize Nulling fraction}
      %\vfill
      \includegraphics[height=7.0cm, width=0.8\textwidth]{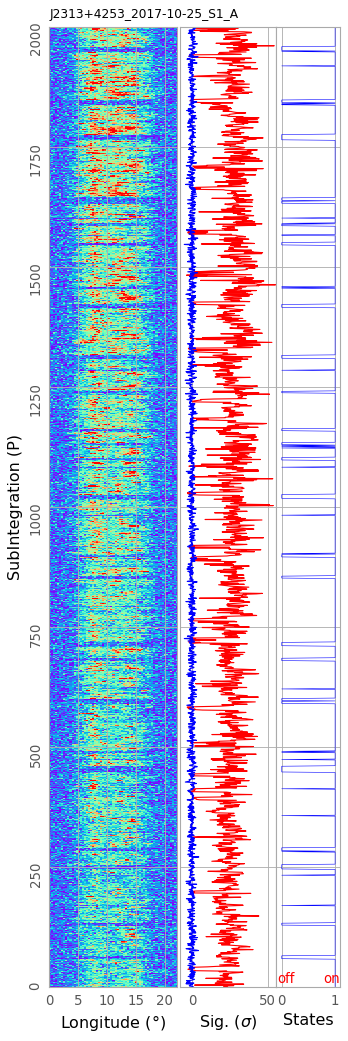}
      \caption{\scriptsize Pulse sequence and states}
      \includegraphics[height=1.0cm,width=0.7\textwidth]{J2313+4253_2017-10-25_S1_A_B_profs.ps}
      \caption{\scriptsize Integrated pulse profiles}
      \vspace{0pt}% reference point at the very bottom
    \end{subfigure}%
  }
  \usebox{\bigimage}
  %\hfill
  \begin{minipage}[b][\ht\bigimage][s]{.2\textwidth}
    \begin{subfigure}{\textwidth}
      \centering
      \includegraphics[height=1.8cm, width=0.8\textwidth]{J2313+4253_2017-10-25_S1_A_BN_dis.ps}
      \caption{\scriptsize Burst and Null lengths}
    \end{subfigure}%
    \vfill
    \begin{subfigure}{\textwidth}
      \centering
      \includegraphics[height=1.8cm, width=0.8\textwidth]{J2313+4253_2017-10-25_S1_A_BN_cor.ps}
      \caption{\scriptsize Brust and Null interaction}
    \end{subfigure}
    \vfill
    \begin{subfigure}{\textwidth}
      \centering
      \includegraphics[height=3.0cm,width=0.7\textwidth]{J2313+4253_2017-10-25_S1_A_BN_period.ps}
      \caption{\scriptsize Nulling periodicity}
    \end{subfigure}
    \vfill
    \begin{subfigure}{\textwidth}
      \centering
      \includegraphics[height=1.7cm,width=0.8\textwidth]{J2313+4253_2017-10-25_S1_A_BE_decay.ps}
      \caption{\scriptsize Variation of burst intensities}
    \end{subfigure}
    \vspace{0pt}% reference point at the very bottom
  \end{minipage}
  \caption{PSR J2313+4253 observed on 2017-10-25A.}
  \label{fig:J2313_20171025A}
\end{figure}
%%%%%%%%%%%%
\begin{figure}
  \centering
  \sbox{\bigimage}{%
    \begin{subfigure}[b]{.2\textwidth}
      \centering
      \includegraphics[height=1.21cm, width=0.8\textwidth]{J2313+4253_2017-10-25_S1_B_NF_dis.ps}
      \caption{\scriptsize Nulling fraction}
      %\vfill
      \includegraphics[height=7.0cm, width=0.8\textwidth]{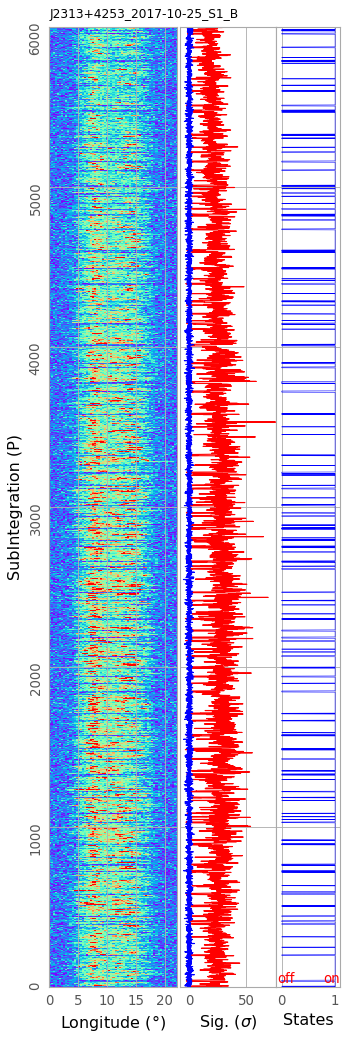}
      \caption{\scriptsize Pulse sequence and states}
      \includegraphics[height=1.0cm,width=0.7\textwidth]{J2313+4253_2017-10-25_S1_B_B_profs.ps}
      \caption{\scriptsize Integrated pulse profiles}
      \vspace{0pt}% reference point at the very bottom
    \end{subfigure}%
  }
  \usebox{\bigimage}
  %\hfill
  \begin{minipage}[b][\ht\bigimage][s]{.2\textwidth}
    \begin{subfigure}{\textwidth}
      \centering
      \includegraphics[height=1.8cm, width=0.8\textwidth]{J2313+4253_2017-10-25_S1_B_BN_dis.ps}
      \caption{\scriptsize Burst and Null lengths}
    \end{subfigure}%
    \vfill
    \begin{subfigure}{\textwidth}
      \centering
      \includegraphics[height=1.8cm, width=0.8\textwidth]{J2313+4253_2017-10-25_S1_B_BN_cor.ps}
      \caption{\scriptsize Brust and Null interaction}
    \end{subfigure}
    \vfill
    \begin{subfigure}{\textwidth}
      \centering
      \includegraphics[height=3.0cm,width=0.7\textwidth]{J2313+4253_2017-10-25_S1_B_BN_period.ps}
      \caption{\scriptsize Nulling periodicity}
    \end{subfigure}
    \vfill
    \begin{subfigure}{\textwidth}
      \centering
      \includegraphics[height=1.7cm,width=0.8\textwidth]{J2313+4253_2017-10-25_S1_B_BE_decay.ps}
      \caption{\scriptsize Variation of burst intensities}
    \end{subfigure}
    \vspace{0pt}% reference point at the very bottom
  \end{minipage}
  \caption{PSR J2313+4253 observed on 2017-10-25B.}
  \label{fig:J2313_20171025B}
\end{figure}
%%%%%%%%%%%%
\begin{figure}
  \centering
  \sbox{\bigimage}{%
    \begin{subfigure}[b]{.2\textwidth}
      \centering
      \includegraphics[height=1.21cm, width=0.8\textwidth]{J2313+4253_2017-10-25_S1_C_NF_dis.ps}
      \caption{\scriptsize Nulling fraction}
      %\vfill
      \includegraphics[height=7.0cm, width=0.8\textwidth]{J2313+4253_2017-10-25_S1_C_Phase_t.ps}
      \caption{\scriptsize Pulse sequence and states}
      \includegraphics[height=1.0cm,width=0.7\textwidth]{J2313+4253_2017-10-25_S1_C_B_profs.ps}
      \caption{\scriptsize Integrated pulse profiles}
      \vspace{0pt}% reference point at the very bottom
    \end{subfigure}%
  }
  \usebox{\bigimage}
  %\hfill
  \begin{minipage}[b][\ht\bigimage][s]{.2\textwidth}
    \begin{subfigure}{\textwidth}
      \centering
      \includegraphics[height=1.8cm, width=0.8\textwidth]{J2313+4253_2017-10-25_S1_C_BN_dis.ps}
      \caption{\scriptsize Burst and Null lengths}
    \end{subfigure}%
    \vfill
    \begin{subfigure}{\textwidth}
      \centering
      \includegraphics[height=1.8cm, width=0.8\textwidth]{J2313+4253_2017-10-25_S1_C_BN_cor.ps}
      \caption{\scriptsize Brust and Null interaction}
    \end{subfigure}
    \vfill
    \begin{subfigure}{\textwidth}
      \centering
      \includegraphics[height=3.0cm,width=0.7\textwidth]{J2313+4253_2017-10-25_S1_C_BN_period.ps}
      \caption{\scriptsize Nulling periodicity}
    \end{subfigure}
    \vfill
    \begin{subfigure}{\textwidth}
      \centering
      \includegraphics[height=1.7cm,width=0.8\textwidth]{J2313+4253_2017-10-25_S1_C_BE_decay.ps}
      \caption{\scriptsize Variation of burst intensities}
    \end{subfigure}
    \vspace{0pt}% reference point at the very bottom
  \end{minipage}
  \caption{PSR J2313+4253 observed on 2017-10-25C.}
  \label{fig:J2313_20171025C}
\end{figure}
%%%%%%%%%%%%
%%%%%%%%%%%%%%%%%%%%%%%%%%%%%%%%%%%%%%%%%%%%%%%%%%%%%%%%%%%%%%%%%%%%%%%%%%%%%%%%%%%%%%%%%%%%%%% J2321
\begin{figure}
  \centering
  \sbox{\bigimage}{%
    \begin{subfigure}[b]{.2\textwidth}
      \centering
      \includegraphics[height=1.21cm, width=0.8\textwidth]{J2321+6024_2015-12-17_S1_0_NF_dis.ps}
      \caption{\scriptsize Nulling fraction}
      %\vfill
      \includegraphics[height=7.0cm, width=0.8\textwidth]{J2321+6024_2015-12-17_S1_0_Phase_t.ps}
      \caption{\scriptsize Pulse sequence and states}
      \includegraphics[height=1.0cm,width=0.7\textwidth]{J2321+6024_2015-12-17_S1_0_B_profs.ps}
      \caption{\scriptsize Integrated pulse profiles}
      \vspace{0pt}% reference point at the very bottom
    \end{subfigure}%
  }
  \usebox{\bigimage}
  %\hfill
  \begin{minipage}[b][\ht\bigimage][s]{.2\textwidth}
    \begin{subfigure}{\textwidth}
      \centering
      \includegraphics[height=1.8cm, width=0.8\textwidth]{J2321+6024_2015-12-17_S1_0_BN_dis.ps}
      \caption{\scriptsize Burst and Null lengths}
    \end{subfigure}%
    \vfill
    \begin{subfigure}{\textwidth}
      \centering
      \includegraphics[height=1.8cm, width=0.8\textwidth]{J2321+6024_2015-12-17_S1_0_BN_cor.ps}
      \caption{\scriptsize Brust and Null interaction}
    \end{subfigure}
    \vfill
    \begin{subfigure}{\textwidth}
      \centering
      \includegraphics[height=3.0cm,width=0.7\textwidth]{J2321+6024_2015-12-17_S1_0_BN_period.ps}
      \caption{\scriptsize Nulling periodicity}
    \end{subfigure}
    \vfill
    \begin{subfigure}{\textwidth}
      \centering
      \includegraphics[height=1.7cm,width=0.8\textwidth]{J2321+6024_2015-12-17_S1_0_BE_decay.ps}
      \caption{\scriptsize Variation of burst intensities}
    \end{subfigure}
    \vspace{0pt}% reference point at the very bottom
  \end{minipage}
  \caption{PSR J2321+6024 observed on 2015-12-17.}
  \label{fig:J2321_20151217}
\end{figure}
%%%%%%%%%%%%
\begin{figure}
  \centering
  \sbox{\bigimage}{%
    \begin{subfigure}[b]{.2\textwidth}
      \centering
      \includegraphics[height=1.21cm, width=0.8\textwidth]{J2321+6024_2017-10-30_S1_A_NF_dis.ps}
      \caption{\scriptsize Nulling fraction}
      %\vfill
      \includegraphics[height=7.0cm, width=0.8\textwidth]{J2321+6024_2017-10-30_S1_A_Phase_t.ps}
      \caption{\scriptsize Pulse sequence and states}
      \includegraphics[height=1.0cm,width=0.7\textwidth]{J2321+6024_2017-10-30_S1_A_B_profs.ps}
      \caption{\scriptsize Integrated pulse profiles}
      \vspace{0pt}% reference point at the very bottom
    \end{subfigure}%
  }
  \usebox{\bigimage}
  %\hfill
  \begin{minipage}[b][\ht\bigimage][s]{.2\textwidth}
    \begin{subfigure}{\textwidth}
      \centering
      \includegraphics[height=1.8cm, width=0.8\textwidth]{J2321+6024_2017-10-30_S1_A_BN_dis.ps}
      \caption{\scriptsize Burst and Null lengths}
    \end{subfigure}%
    \vfill
    \begin{subfigure}{\textwidth}
      \centering
      \includegraphics[height=1.8cm, width=0.8\textwidth]{J2321+6024_2017-10-30_S1_A_BN_cor.ps}
      \caption{\scriptsize Brust and Null interaction}
    \end{subfigure}
    \vfill
    \begin{subfigure}{\textwidth}
      \centering
      \includegraphics[height=3.0cm,width=0.7\textwidth]{J2321+6024_2017-10-30_S1_A_BN_period.ps}
      \caption{\scriptsize Nulling periodicity}
    \end{subfigure}
    \vfill
    \begin{subfigure}{\textwidth}
      \centering
      \includegraphics[height=1.7cm,width=0.8\textwidth]{J2321+6024_2017-10-30_S1_A_BE_decay.ps}
      \caption{\scriptsize Variation of burst intensities}
    \end{subfigure}
    \vspace{0pt}% reference point at the very bottom
  \end{minipage}
  \caption{PSR J2321+6024 observed on 2017-10-30A.}
  \label{fig:J2321_20171030A}
\end{figure}
%%%%%%%%%%%%
\begin{figure}
  \centering
  \sbox{\bigimage}{%
    \begin{subfigure}[b]{.2\textwidth}
      \centering
      \includegraphics[height=1.21cm, width=0.8\textwidth]{J2321+6024_2017-10-30_S1_B_NF_dis.ps}
      \caption{\scriptsize Nulling fraction}
      %\vfill
      \includegraphics[height=7.0cm, width=0.8\textwidth]{J2321+6024_2017-10-30_S1_B_Phase_t.ps}
      \caption{\scriptsize Pulse sequence and states}
      \includegraphics[height=1.0cm,width=0.7\textwidth]{J2321+6024_2017-10-30_S1_B_B_profs.ps}
      \caption{\scriptsize Integrated pulse profiles}
      \vspace{0pt}% reference point at the very bottom
    \end{subfigure}%
  }
  \usebox{\bigimage}
  %\hfill
  \begin{minipage}[b][\ht\bigimage][s]{.2\textwidth}
    \begin{subfigure}{\textwidth}
      \centering
      \includegraphics[height=1.8cm, width=0.8\textwidth]{J2321+6024_2017-10-30_S1_B_BN_dis.ps}
      \caption{\scriptsize Burst and Null lengths}
    \end{subfigure}%
    \vfill
    \begin{subfigure}{\textwidth}
      \centering
      \includegraphics[height=1.8cm, width=0.8\textwidth]{J2321+6024_2017-10-30_S1_B_BN_cor.ps}
      \caption{\scriptsize Brust and Null interaction}
    \end{subfigure}
    \vfill
    \begin{subfigure}{\textwidth}
      \centering
      \includegraphics[height=3.0cm,width=0.7\textwidth]{J2321+6024_2017-10-30_S1_B_BN_period.ps}
      \caption{\scriptsize Nulling periodicity}
    \end{subfigure}
    \vfill
    \begin{subfigure}{\textwidth}
      \centering
      \includegraphics[height=1.7cm,width=0.8\textwidth]{J2321+6024_2017-10-30_S1_B_BE_decay.ps}
      \caption{\scriptsize Variation of burst intensities}
    \end{subfigure}
    \vspace{0pt}% reference point at the very bottom
  \end{minipage}
  \caption{PSR J2321+6024 observed on 2017-10-30B.}
  \label{fig:J2321_20171030B}
\end{figure}
%%%%%%%%%%%%
\begin{figure}
  \centering
  \sbox{\bigimage}{%
    \begin{subfigure}[b]{.2\textwidth}
      \centering
      \includegraphics[height=1.21cm, width=0.8\textwidth]{J2321+6024_2017-10-30_S1_C_NF_dis.ps}
      \caption{\scriptsize Nulling fraction}
      %\vfill
      \includegraphics[height=7.0cm, width=0.8\textwidth]{J2321+6024_2017-10-30_S1_C_Phase_t.ps}
      \caption{\scriptsize Pulse sequence and states}
      \includegraphics[height=1.0cm,width=0.7\textwidth]{J2321+6024_2017-10-30_S1_C_B_profs.ps}
      \caption{\scriptsize Integrated pulse profiles}
      \vspace{0pt}% reference point at the very bottom
    \end{subfigure}%
  }
  \usebox{\bigimage}
  %\hfill
  \begin{minipage}[b][\ht\bigimage][s]{.2\textwidth}
    \begin{subfigure}{\textwidth}
      \centering
      \includegraphics[height=1.8cm, width=0.8\textwidth]{J2321+6024_2017-10-30_S1_C_BN_dis.ps}
      \caption{\scriptsize Burst and Null lengths}
    \end{subfigure}%
    \vfill
    \begin{subfigure}{\textwidth}
      \centering
      \includegraphics[height=1.8cm, width=0.8\textwidth]{J2321+6024_2017-10-30_S1_C_BN_cor.ps}
      \caption{\scriptsize Brust and Null interaction}
    \end{subfigure}
    \vfill
    \begin{subfigure}{\textwidth}
      \centering
      \includegraphics[height=3.0cm,width=0.7\textwidth]{J2321+6024_2017-10-30_S1_C_BN_period.ps}
      \caption{\scriptsize Nulling periodicity}
    \end{subfigure}
    \vfill
    \begin{subfigure}{\textwidth}
      \centering
      \includegraphics[height=1.7cm,width=0.8\textwidth]{J2321+6024_2017-10-30_S1_C_BE_decay.ps}
      \caption{\scriptsize Variation of burst intensities}
    \end{subfigure}
    \vspace{0pt}% reference point at the very bottom
  \end{minipage}
  \caption{PSR J2321+6024 observed on 2017-10-30C.}
  \label{fig:J2321_20171030C}
\end{figure}
%%%%%%%%%%%%
%%%%%%%%%%%%
%\clearpage
%%%%%%%%%%%%
\begin{figure}
  \centering
  \sbox{\bigimage}{%
    \begin{subfigure}[b]{.2\textwidth}
      \centering
      \includegraphics[height=1.21cm, width=0.8\textwidth]{J2321+6024_2017-10-30_S1_D_NF_dis.ps}
      \caption{\scriptsize Nulling fraction}
      %\vfill
      \includegraphics[height=7.0cm, width=0.8\textwidth]{J2321+6024_2017-10-30_S1_D_Phase_t.ps}
      \caption{\scriptsize Pulse sequence and states}
      \includegraphics[height=1.0cm,width=0.7\textwidth]{J2321+6024_2017-10-30_S1_D_B_profs.ps}
      \caption{\scriptsize Integrated pulse profiles}
      \vspace{0pt}% reference point at the very bottom
    \end{subfigure}%
  }
  \usebox{\bigimage}
  %\hfill
  \begin{minipage}[b][\ht\bigimage][s]{.2\textwidth}
    \begin{subfigure}{\textwidth}
      \centering
      \includegraphics[height=1.8cm, width=0.8\textwidth]{J2321+6024_2017-10-30_S1_D_BN_dis.ps}
      \caption{\scriptsize Burst and Null lengths}
    \end{subfigure}%
    \vfill
    \begin{subfigure}{\textwidth}
      \centering
      \includegraphics[height=1.8cm, width=0.8\textwidth]{J2321+6024_2017-10-30_S1_D_BN_cor.ps}
      \caption{\scriptsize Brust and Null interaction}
    \end{subfigure}
    \vfill
    \begin{subfigure}{\textwidth}
      \centering
      \includegraphics[height=3.0cm,width=0.7\textwidth]{J2321+6024_2017-10-30_S1_D_BN_period.ps}
      \caption{\scriptsize Nulling periodicity}
    \end{subfigure}
    \vfill
    \begin{subfigure}{\textwidth}
      \centering
      \includegraphics[height=1.7cm,width=0.8\textwidth]{J2321+6024_2017-10-30_S1_D_BE_decay.ps}
      \caption{\scriptsize Variation of burst intensities}
    \end{subfigure}
    \vspace{0pt}% reference point at the very bottom
  \end{minipage}
  \caption{PSR J2321+6024 observed on 2017-10-30D.}
  \label{fig:J2321_20171030D}
\end{figure}
%%%%%%%%%%%%
